# Supplementary material for: Online learning in bandits with predicted context
Source: arXiv:2307.13916 source file (2024-03-18)
Supplement: Supplementary file 1 [file appendix.tex]

\section{Additional simulations}\label{appendix-simulation+}

%\subsection{{\color{red} Real data}}

\subsection{Improving early stage performance of \texttt{MEB}: an example}

In Section \ref{section:simulations}, we mentioned that the performance of \texttt{MEB} in the early stage can be improved by several potential methods. In this section, we show some preliminary simulation results of one simple variant of \texttt{MEB}: Instead of always making decisions with (\ref{eq:proposed-estimator}), in the first $T_1$ rounds after the pure exploration, we use the estimator $\hat\btheta_{a, me}^{(t)}$ from (\ref{eq:naive-estimator}) to make the decision. That is to say, for $t = T_0+1, \ldots, T_1$, we modify line 7 of Algorithm \ref{alg1} to 
$$
\tilde a_t \leftarrow \argmax_{a\in\{0, 1\}}\langle\hat\btheta_{a, me}^{(t)}, \tilde\xb_t\rangle.
$$
It is easy to see that both the estimation and regret guarantees remain valid as long as $T_1 = \cO(1)$. In fact, we can also replace (\ref{eq:naive-estimator}) with any estimator that achieves empirically good early-stage performance. Below, we compare this newly proposed variant, \texttt{MEB-naive-init}, to the three algorithms shown in Section \ref{section:simulations} in terms of the early-stage empirical performance (up to $t=10000$) under the same settings of Section \ref{section:simulations}.

\begin{figure}[h]
\centering
\includegraphics[width=1.0\textwidth]{meb_init.pdf}
\caption{Estimation error ($\|\hat\btheta_0^{(t)}-\btheta_0^*\|_2$) and cumulative regret of four algorithms with minimum exploration probability $p_0 = 0.1$ and $p_0 = 0.01$ under the settings of normal and heavy-tailed errors $(\bepsilon_t)_{t\geq 1}$. The results are calculated from $n_{exp}=500$ independent experiments. The red, blue, green, and black line corresponds to Thompson sampling, \texttt{MEB} (Algorithm \ref{alg1}), \texttt{MEB-naive} (Algorithm \ref{alg1} plugged in with the naive measurement error estimator (\ref{eq:naive-estimator})), and \texttt{MEB-naive-init} (Algorithm \ref{alg1} plugged in with the naive measurement error estimator (\ref{eq:naive-estimator}) up to time $t=2000$, and (\ref{eq:proposed-estimator}) afterward) respectively. The solid lines indicate the mean values, while the shaded bands represent the standard errors across the independent experiments.}
\label{fig:meb_init}
\end{figure}

Figure \ref{fig:meb_init} shows the estimation error (for $\btheta_0^*$) as well as the cumulative regret of the four algorithms with two choices of $p_0$ under different settings of $\bepsilon_t$ distributions. Here, in \texttt{MEB-naive-init}, we use the naive estimator up to round 2000, and then continue to use our proposed estimator (\ref{eq:proposed-estimator}) for decision-making. We can see that in all the settings we consider here, \texttt{MEB-naive-init} not only decreases the estimation error as desired, but also significantly improves the cumulative regret performance compare to \texttt{MEB} due to making better decisions early in the algorithm. This improvement is especially significant when the minimum sampling probability, $p_0$, is small. After 2000 rounds, \texttt{MEB-naive-init} is able to make decisions of the same quality as \texttt{MEB}. In practice, we can also tune $T_1$, or explore other estimators when $t\leq T_1$ to further improve the performance.  %\sam{we should comment that as the number of examples increases, MEB  end up with lower regret compared to both MEB naive and MEB naive init. Right now our language appears to indicate that MEB naive init is always better. }

As mentioned in Section \ref{section:simulations}, \texttt{MEB-naive-init} is not the only way to boost the early performance of \texttt{MEB} due to the enlarged variance caused by importance weights. The alternative approaches (e.g. variance reduction techniques, fine-tuning the sampling rate $(p_0^{(t)})_{t\geq 1}$) are left for further investigation and are not explored in detail in this paper.

\subsection{{Results for different magnitudes of measurement error}}

\begin{figure}[h]
\centering
\includegraphics[width=1.0\textwidth]{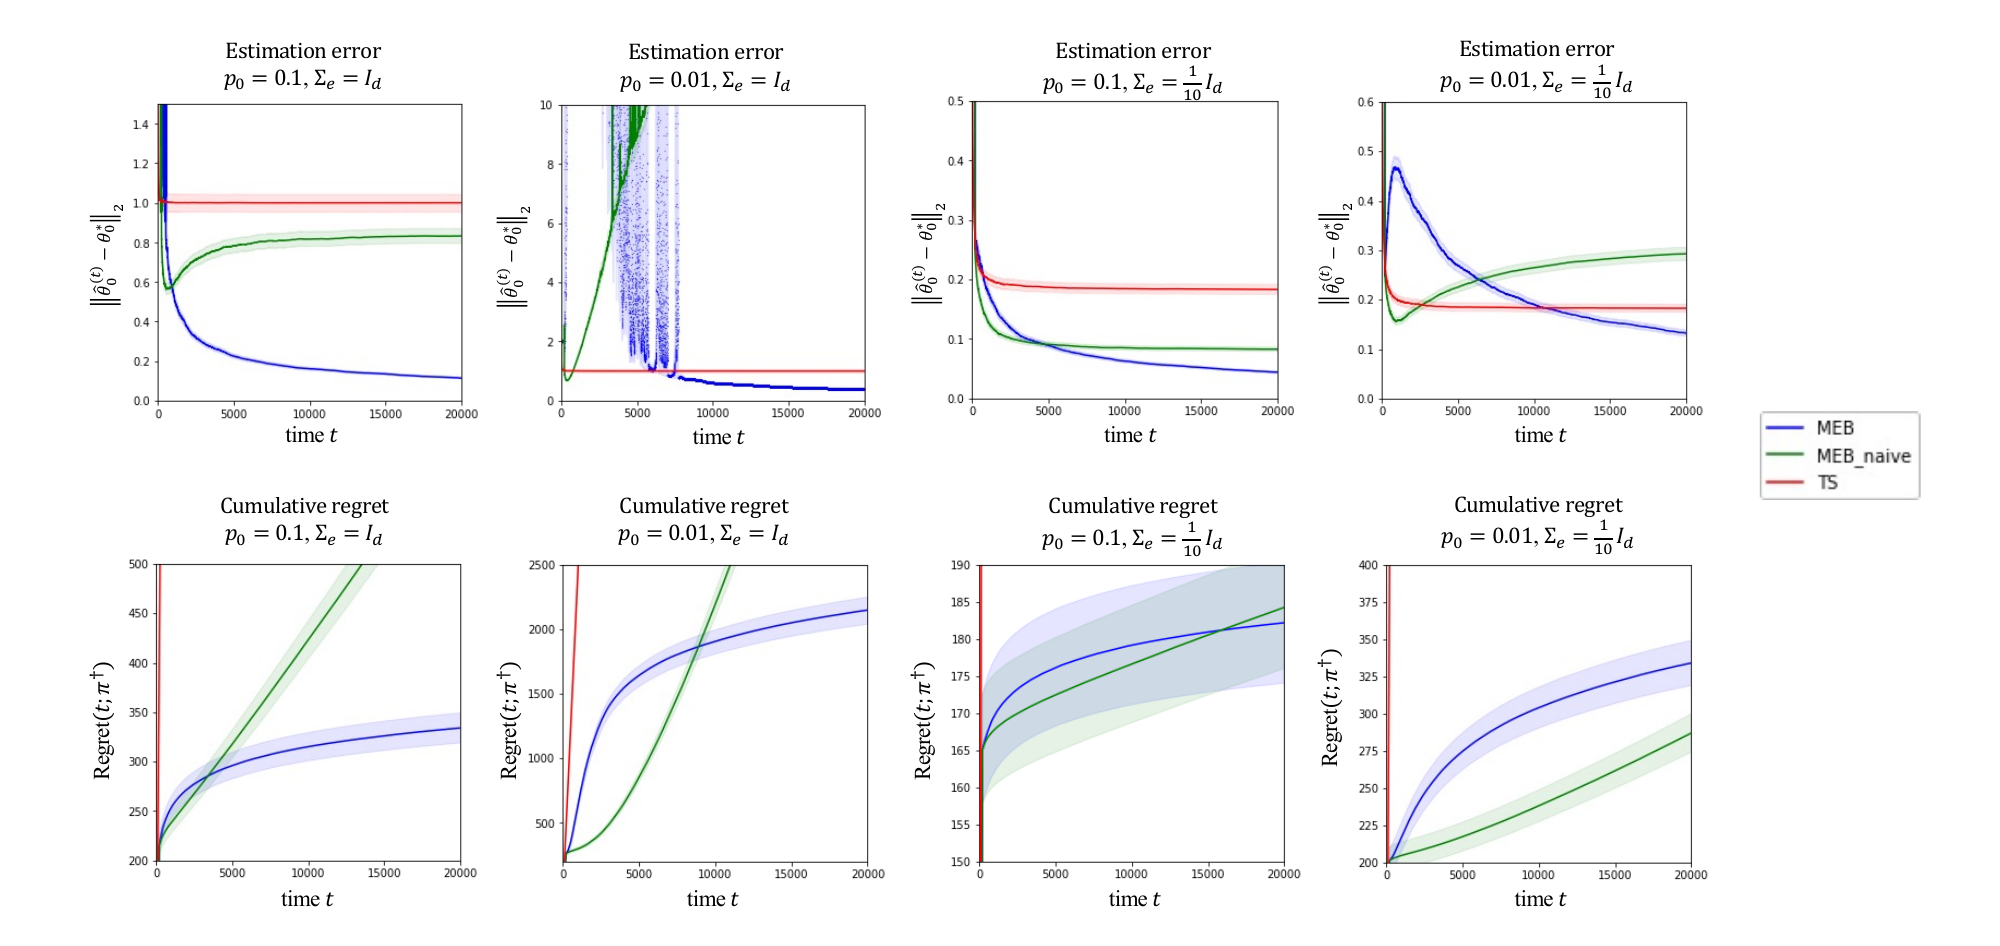}
\caption{Estimation error ($\|\hat\btheta_0^{(t)}-\btheta_0^*\|_2$) and cumulative regret of three algorithms with minimum exploration probability $p_0=0.1$ and $p_0 = 0.01$, when the error variance $\bSigma_e = \bI_d$ and $\bSigma_e = 0.1\cdot \bI_d$. The results are calculated from $n_{exp} = 500$ independent experiments. The red, green, and blue line corresponds to Thompson sampling, \texttt{MEB} (Algorithm \ref{alg1}), and \texttt{MEB-naive} (\texttt{MEB} plugged in with the naive estimator (\ref{eq:naive-estimator})) respectively. The solid lines indicate the mean values, while the shaded bands represent the standard errors across the independent experiments.}
\label{fig:simulation_different_me_size}
\end{figure}

We provide additional simulation results under the same setting of Section \ref{section:simulations} but with different magnitudes of the errors $\bepsilon_t$. Specifically, Figure \ref{fig:simulation_different_me_size} shows the estimation error ($\|\hat\btheta_0^{(t)}-\btheta_0^*\|_2$) as well as the cumulative regret of Thompson sampling, \texttt{MEB} and \texttt{MEB-naive} with minimum sampling probability $p_0 = 0.1$ and $p_0 = 0.01$
when $\bepsilon_t\sim \cN(\mathbf{0}, \bSigma_e)$, $\bSigma_e = \bI_d$ and $0.1\cdot \bI_d$ (recall that in section \ref{section:simulations}, we did simulations for $\bSigma_e = 0.25\cdot \bI_d$). In general, larger $\bSigma_e$ makes the problem more difficult. $\bSigma_e = \bI_d$ and $p_0 = 0.01$ is actually a pretty extreme case since the large variation of $\bepsilon_t$ and small sampling probability will make the measurement error estimators numerically unstable (Note that the true context $\xb_t\sim\cN(\mathbf{1}_d, \bI_d)$).

Despite the different levels of $\bSigma_e$, we observe similar findings as in Section \ref{section:simulations}: \texttt{MEB} is the only algorithm that leads to sublinear regret and produces estimators that converge to the ground truth. Even in the extreme case ($\bSigma_e=\bI_d$, $p_0 = 0.01$) where the estimator (\ref{eq:proposed-estimator}) is unstable during the early stages of the algorithm, it has little impact on the quality of the decisions, as the regret curve stops growing fast way before the estimation error starts to stabilize. In addition, as previously mentioned, we can also warm start \texttt{MEB} to boost its performance during the early stages. 

All the computational results are performed on a MacBook Pro (Apple M1 chip, 8GB Memory) and an iMac (Apple M1 chip, 8GB Memory).

\section{Example: inconsistency of the naive estimator (\ref{eq:naive-estimator})}\label{appendix-failure-of-naive-estimator}

\begin{example}\label{ex:failure-of-naive-estimator}
Let $d = 1$, $\xb_{\tau}\equiv 1$ for all ${\tau}$, and $\bepsilon_{\tau}\sim \text{Unif}(-2, 2)$ sampled independently. For the reward model, let $\btheta_0^* = -1$, $\btheta_1^*= 1$, $\eta_{\tau}\sim \text{Unif}(-0.1, 0.1)$ sampled independently. So in order to maximize expected reward, we should choose action 1 if $\xb_{\tau}$ is positive and action 0 otherwise. Suppose the agent takes the following policy that is stationary and non-adaptive to history:  
$$
\pi_{\tau}(A)=
\begin{cases}
\frac{2}{3}1_{\{A = 1\}} + \frac{1}{3}1_{\{A = 0\}},\quad\text{if }\tilde\xb_{\tau}
%= \xb_{\tau}+\bepsilon_{\tau}
>\rho \\
\frac{1}{3}1_{\{A = 1\}} + \frac{2}{3}1_{\{A = 0\}},\quad\text{otherwise.}
\end{cases}
$$
Here, $\rho$ is a pre-specified  constant. Figure \ref{fig:theta_estimation} (a) plots the mean and standard deviation of $\hat\btheta_{0, me}^{(t)}$ (as in (\ref{eq:naive-estimator})) given 100 independent experiments for each $t=1,\ldots, 10000$, where $\rho = -0.5, 0, 0.5$. Observe that as $t$ grows, $\hat\btheta_{0, me}^{(t)}$ 
converges to different limits for different policies. In general, 
the limit is not equal to $\btheta_0^* = -1$.

In contrast, Figure \ref{fig:theta_estimation} (b) shows the mean and standard deviation of $\hat\btheta_0^{(t)}$ (as in (\ref{eq:proposed-estimator})) given 100 independent experiments under the same setting with the same three policies as in Figure \ref{fig:theta_estimation} (a). Unlike the naive estimator (\ref{eq:naive-estimator}), the proposed estimator (\ref{eq:proposed-estimator}) quickly converges around the true value $-1$ for all three candidate policies.
\end{example}

\begin{figure}[h]
\centering
\includegraphics[width=1.0\textwidth]{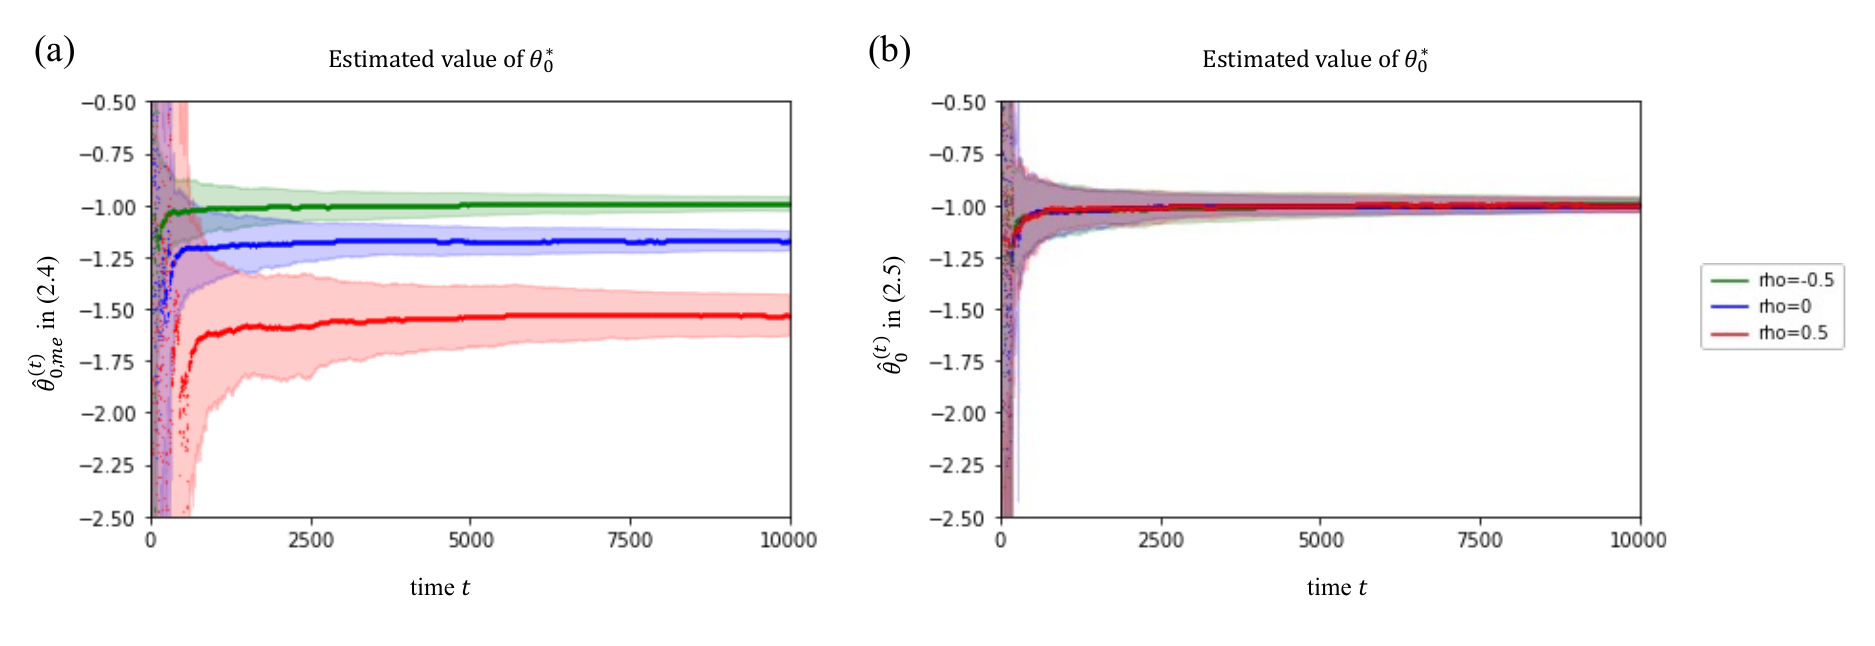}
\caption{Estimated value of $\btheta_0^*$ given the naive estimator (\ref{eq:naive-estimator}) in (a) and our proposed estimator (\ref{eq:proposed-estimator}) in (b) under different policies under 100 independent experiments. The green, blue, and red line corresponds to the policy with parameter $\rho = -0.5, 0$, and $0.5$ respectively. The solid lines indicate the mean values, while the shaded bands represent the standard deviation across the independent experiments.}
\label{fig:theta_estimation}
\end{figure}

\section{Regret guarantees compare to the standard benchmark policy (\ref{eq:nonclipped-oracle-policy})}\label{appendix:usual-benchmark}

In this section, we provide theoretical guarantees that by choosing other hyperparameter values, \texttt{MEB} can achieve regret $\cO(T^{2/3})$ compared to the standard benchmark $\pi^*$. %The proof is in subsection \ref{pf:thm:standard-benchmark}.

\begin{theorem}\label{thm:standard-benchmark}
Under Assumptions \ref{ass:boundedness} and \ref{ass:min-signal}, there exist constants $C$ and $C_1$ such that by choosing $T_0 = \lceil 2 T^{\frac23}\rceil$, $p_0^{(t)} = t^{-\frac13}$, for any $T$ satisfying $T\geq C_1\max\{1, (d+\log T)^{\frac94}, \big(\frac{d+\log T}{\lambda_0\wedge\lambda_0^2}\big)^{\frac94}\}$, with probability at least $1-\frac{16}{\sqrt{T}}$, the regret of Algorithm \ref{alg1}:
$$
\text{Regret}(T;\pi^*)\leq C\left\{R_\theta T^{\frac23}+\frac{R+R_\theta}{\lambda_0}T^{\frac23}\sqrt{d+\log T}\right\}.
$$
\end{theorem}
%\sam{usually in regret bounds we set the probability to be at least $1-\delta$ for $\delta$ a constant.   But above the prob is at least $1-16/\sqrt{T}$.  This makes it hard to understand the results.   Can you make the probability lower bound be $1-\delta$?}

%\sam{Also it is a little odd to separate the theorem from the proof when in the appendix.  I would put them together...}

%\subsection{Proof of Theorem \ref{thm:standard-benchmark}}\label{pf:thm:standard-benchmark}
\begin{proof}
First, notice that $q_t = \min_{\tau\leq t, a\in\{0, 1\}}\pi_\tau(a|\tilde\xb_t, \cH_{\tau-1}) = p_0^{(t)}$, since $p_0^{(t)}$ is monotonically decreasing in $t$. Theorem \ref{thm:theta-estimation} indicates that, as long as 
\begin{equation}\label{eq:standard-benchmark-condition1}
p_0^{(t)}\geq \frac{C_1}{\lambda_0\wedge\lambda_0^2}\frac{d+\log t}{t},
\end{equation}
with probability at least $1-\frac{8}{t^2}$, for any $a\in\{0, 1\}$
\begin{equation}\label{eq:standard-benchmark-estimation-error}
\|\hat\btheta_a^{(t)}-\btheta_a^*\|_2
\leq \frac{C(R+R_\theta)}{\lambda_0}\max\left\{\frac{d+\log t}{t^{\frac23}}, \sqrt{\frac{d+\log t}{t^{\frac23}}}\right\}.
\end{equation}

At any time $t>T_0$, the instantaneous regret can be controlled by 
\begin{align}
{\text{Regret}}_t^* &= \EE_{a\sim \pi_t^*}\langle \btheta^*_{a}, \tilde\xb_t\rangle - \EE_{a\sim \pi_t}\langle \btheta^*_{a}, \tilde\xb_t\rangle\nonumber\\
&=\langle\btheta^*_{a_t^\dagger}, \tilde\xb_t\rangle-[(1-p_0^{(t)})\langle\btheta^*_{\tilde a_t}, \tilde\xb_t\rangle+p_0^{(t)}\langle\btheta^*_{1-\tilde a_t}, \tilde\xb_t\rangle]\nonumber\\
&= 1_{\{a_t^\dagger= \tilde a_t\}}p_0^{(t)}\langle \btheta^*_{a_t^\dagger} - \btheta^*_{1-a_t^\dagger}, \tilde\xb_t\rangle + 1_{\{a_t^\dagger\neq \tilde a_t\}}(1-p_0^{t})\langle \btheta^*_{a_t^\dagger} - \btheta^*_{1-a_t^\dagger}, \tilde\xb_t\rangle\nonumber\\
&\leq 2p_0^{(t)}R_\theta + 1_{\{a_t^\dagger\neq \tilde a_t\}}\langle \btheta^*_{a_t^\dagger} - \btheta^*_{1-a_t^\dagger}, \tilde\xb_t\rangle.\label{eq:instant-regret-standard-benchmark}
\end{align}
Here recall that $a_t^\dagger:=\argmax_a\langle \btheta^*_{a}, \tilde\xb_t\rangle$, $\tilde a_t := \argmax_{a\in\{0, 1\}}\langle\hat\btheta_{a}^{(t-1)}, \tilde\xb_t\rangle$.

Note that $a_t^\dagger\neq \tilde a_t$ implies that 
\begin{align*}
\begin{cases}
\langle\btheta_{a_t^\dagger}^*, \tilde\xb_t\rangle\geq \langle\btheta_{1-a_t^\dagger}^*, \tilde\xb_t\rangle\\
\langle\hat\btheta_{a_t^\dagger}^{(t-1)}, \tilde\xb_t\rangle\leq \langle\hat\btheta_{1-a_t^\dagger}^{(t-1)}, \tilde\xb_t\rangle
\end{cases}
\end{align*}
which leads to 
\begin{align*}
\langle \btheta_{a_t^\dagger}^*, \tilde\xb_t\rangle&\geq \langle\btheta_{1-a_t^\dagger}^*, \tilde\xb_t\rangle\geq \langle\hat\btheta_{1-a_t^\dagger}^{(t-1)}, \tilde\xb_t\rangle - \max_a\|\hat\btheta_a^{(t-1)}-\btheta_a^*\|_2\\
&\geq \langle\hat\btheta_{a_t^\dagger}^{(t-1)}, \tilde\xb_t\rangle - \max_a\|\hat\btheta_a^{(t-1)}-\btheta_a^*\|_2\geq \langle\btheta_{a_t^\dagger}^*, \tilde\xb_t\rangle - 2\max_a\|\hat\btheta_a^{(t-1)}-\btheta_a^*\|_2,
\end{align*}
and further implies $\left|\langle \btheta^*_{a_t^\dagger} - \btheta^*_{1-a_t^\dagger}, \tilde\xb_t\rangle\right|\leq 2\max_a\|\hat\btheta_a^{(t-1)}-\btheta_a^*\|_2$.

Plugging in the above to (\ref{eq:instant-regret-standard-benchmark}) leads to an upper bound of instantaneous regret
\begin{align*}
\text{Regret}_t^*&\leq 2p_0^{(t)}R_\theta + 2\max_a\|\hat\btheta_a^{(t-1)}-\btheta_a^*\|_2 \\
&\leq \frac{2R_\theta}{t^{\frac13}} + 
\frac{2C(R+R_\theta)}{\lambda_0}\max\left\{\frac{d+\log (t-1)}{(t-1)^{\frac23}}, \sqrt{\frac{d+\log (t-1)}{(t-1)^{\frac23}}}\right\}\\
&\leq \frac{2R_\theta}{t^{\frac13}} + \frac{2C(R+R_\theta)}{\lambda_0}\max\left\{\frac{d+\log t}{(t/2)^{\frac23}}, \sqrt{\frac{d+\log t}{(t/2)^{\frac23}}}\right\}\\
&\leq \frac{2R_\theta}{t^{\frac13}} + \frac{4C(R+R_\theta)}{\lambda_0}\max\left\{\frac{d+\log t}{t^{\frac23}}, \sqrt{\frac{d+\log t}{t^{\frac23}}}\right\}
\end{align*}
for $t>T_0$. If in addition, for all $t\geq T_0$,
\begin{equation}\label{eq:standard-benchmark-condition2}
\frac{d+\log t}{t^{\frac23}}\leq 1,
\end{equation}
then we further have
\begin{align*}
\text{Regret}_t^*
&\leq \frac{2R_\theta}{t^{\frac13}} + \frac{4C(R+R_\theta)}{\lambda_0}\sqrt{\frac{d+\log t}{t^{\frac23}}}
\end{align*}
for $t>T_0$. Meanwhile, notice that $\text{Regret}_t^*\leq 2R_\theta$ for any $t\leq T_0$. Thus, we deduce that the cumulative regret compared to the standard benchmark:
\begin{align}
\text{Regret}(T;\pi^*)
&\leq T_0\cdot 2R_\theta + \sum_{t>2T^{\frac23}}\left(2R_\theta t^{-\frac13}+\frac{4C(R+R_\theta)}{\lambda_0}t^{-\frac13}\sqrt{d+\log t}\right)\nonumber\\
&\leq C_2\left\{R_\theta T^{\frac23} + \frac{R+R_\theta}{\lambda_0}T^{\frac23}\sqrt{d+\log T}\right\}
\end{align}
For a universal constant $C_2$. Finally, conditions (\ref{eq:standard-benchmark-condition1}) and (\ref{eq:standard-benchmark-condition2}) can be guaranteed by $T\geq C_3\max\{1, (d+\log T)^{\frac94}, \big(\frac{d+\log T}{\lambda_0\wedge\lambda_0^2}\big)^{\frac94}\}$ for some universal constant $C_3$.
\end{proof}

\section{Generalization to $K\geq 2$ actions} \label{appendix:generalization-to-K-actions}

In this section, we assume that $\cA = \{1, 2, \ldots, K\}$ instead of $\{0, 1\}$. The benchmarks (\ref{eq:nonclipped-oracle-policy}) and (\ref{eq:oracle-policy}) become
\begin{equation}\label{eq:standard-benchmark-multiple-actions}
\pi_t^*(a) = 
\begin{cases}
1,\quad &\text{if }a = a_t^\dagger = \argmax_a\langle\btheta_a^*, \tilde \xb_t\rangle\\
0,\quad &\text{otherwise, }
\end{cases}
\end{equation}
and 
\begin{equation}\label{eq:clipped-benchmark-multiple-actions}
\pi_t^\dagger(a) = 
\begin{cases}
1-(K-1)p_0,\quad &\text{if }a = a_t^\dagger = \argmax_a\langle\btheta_a^*, \tilde \xb_t\rangle\\
p_0,\quad &\text{otherwise. }
\end{cases}
\end{equation}

In the $K$-arm setting, we can still estimate $\btheta_a^*$ using (\ref{eq:proposed-estimator}) for each $a\in\cA$. Using the same proof ideas as Theorem \ref{thm:theta-estimation}, we can get the following theoretical guarantees (proof omitted):

\begin{theorem}[Corresponds to Theorem \ref{thm:theta-estimation}]\label{thm:theta-estimation-multiple-actions}
For any $t\in[T]$, let $q_t = \inf_{\tau\in[t], a\in\cA}\pi_\tau(a|\tilde\xb_\tau, \cH_{\tau-1})$. Then under Assumptions \ref{ass:boundedness} and \ref{ass:min-signal}, there exist constants $C$ and $C_1$ such that as long as $q_t\geq \frac{C_1}{\lambda_0\wedge\lambda_0^2}\frac{d+\log t}{t}$, with probability at least $1-\frac{4K}{t^2}$,
$$
\|\hat\btheta_a^{(t)}-\btheta_a^*\|_2\leq \frac{C(R+R_\theta)}{\lambda_0}\max\left\{\frac{d+\log t}{q_tt}, \sqrt{\frac{d+\log t}{q_tt}}\right\}, \quad \forall a\in\cA.
$$
\end{theorem}

\setcounter{algorithm}{1}
\begin{algorithm}[t]
	\caption{\texttt{MEB} with $K$ actions}	
	\label{alg1-multiple-actions}
	\begin{algorithmic}[1]		
\STATE \textbf{{Input}}: $(\bSigma_{e, t})_{t\in[T]}$: covariance sequence of $(\bepsilon_t)_{t\in[T]}$; $(p_0^{(t)})_{t\in[T]}$: minimum selection probability at each time $t$; $T_0$: length of pure exploration
        \FOR{time $t = 1, 2, \ldots, T$}
        \IF{$t\leq T_0$}
        \STATE Sample $a_t\sim \pi_t(\cdot|\tilde\xb_t, \cH_{t-1})$, where $\pi_t(a|\tilde\xb_t, \cH_{t-1}) = 1/K$ for all $a\in\cA$
        \ELSE
        \STATE Obtain updated estimators $(\hat\btheta_{a}^{(t-1)})_{a\in\cA}$ from (2.6)
        \STATE $\tilde a_t \leftarrow \argmax_{a\in\cA}\langle\hat\btheta_{a}^{(t-1)}, \tilde\xb_t\rangle$
        \STATE Sample $a_t\sim \pi_t(\cdot|\tilde\xb_t, \cH_{t-1})$, where $\pi_t(a|\tilde\xb_t, \cH_{t-1}):=
        \begin{cases}
        1-(K-1)p_{0}^{(t)}, \quad\text{if }a = \tilde a_t\\
        p_{0}^{(t)}, \quad\text{otherwise}
        \end{cases}
        $
        \ENDIF
        \ENDFOR
	\end{algorithmic}
\end{algorithm}

\texttt{MEB} with $K$ actions is shown in Algorithm \ref{alg1-multiple-actions}. When compared to the benchmark (\ref{eq:clipped-benchmark-multiple-actions}), as in Theorem \ref{thm-regret}, we can still control its regret by the estimation error of (\ref{eq:proposed-estimator}). See the Theorem below (The proof is only slightly different from Theorem \ref{thm-regret}; We briefly list it in Appendix \ref{pf:thm:regret-multiple-actions}).

\begin{theorem}[Corresponds to Theorem \ref{thm-regret}]\label{thm:regret-multiple-actions}
Given Assumption \ref{ass:boundedness}, the regret of Algorithm \ref{alg1-multiple-actions} satisfies
$$
\text{Regret}(T;\pi^\dagger)\leq 2T_0R_\theta+2(1-Kp_0)\sum_{t\in(T_0, T]}\max_{a\in\cA}\|\btheta_a^{(t-1)} - \btheta_a^*\|_2.
$$
\end{theorem}

Combining Theorems \ref{thm:theta-estimation-multiple-actions} and \ref{thm:regret-multiple-actions}, we obtain the following corollary. Its proof is the same as Corollary \ref{cor:alg1-with-theta-estimation}, and is thus omitted.

\begin{corollary}[Corresponds to Corollary \ref{cor:alg1-with-theta-estimation}]\label{cor:alg1-with-theta-estimation-multiple-actions}
There exist constants $C$, $C'$ such that by choosing $T_0 = \lceil 2\sqrt{T}\rceil$, for any $T$ satisfying $T\geq C'\max\{1, \frac{d^2+\log ^2(T)}{p_0^2}, \frac{d^2+\log^2(T)}{\lambda_0^2(1\wedge\lambda_0^2)p_0^2}\}$, with probability at least $1-\frac{8K}{\sqrt{T}}$, the regret of Algorithm \ref{alg1-multiple-actions}:
$$
\text{Regret}(T;\pi^\dagger)\leq C\left\{R_\theta\sqrt{T} + \frac{(R+R_\theta)(1-Kp_0)}{\lambda_0\sqrt{p_0}}\sqrt{T(d+\log T)}\right\}.
$$
\end{corollary}

Finally, compared to the benchmark (\ref{eq:standard-benchmark-multiple-actions}), we have the following regret guarantees (Proof in Appendix \ref{pf:thm:standard-benchmark-multiple-actions}).

\begin{theorem}\label{thm:standard-benchmark-multiple-actions}
Under Assumptions \ref{ass:boundedness} and \ref{ass:min-signal}, there exist constants $C$ and $C_1$ such that by choosing $T_0 = \lceil 2T^{\frac23}\rceil$, $p_0^{(t)} = t^{-\frac13}$ in Algorithm \ref{alg1-multiple-actions}, for any $T$ satisfying $T\geq C_1\max\{1, (d+\log T)^{\frac94}, \big(\frac{d+\log T}{\lambda_0\wedge\lambda_0^2}\big)^{\frac94}\}$, with probability at least $1-\frac{8K}{\sqrt{T}}$, the regret of Algorithm \ref{alg1-multiple-actions}:
$$
\text{Regret}(T;\pi^*) \leq C\left\{(K-1)R_\theta T^{\frac23}+\frac{R+R_\theta}{\lambda_0}T^{\frac23}\sqrt{d+\log T}\right\}.
$$
\end{theorem}

\section{Justification of the benchmark policy (Proof of Lemma \ref{lem:oracle})}\label{pf:lem:oracle}

We first prove (i). When $\langle\btheta_0^*-\btheta_{1}^*, \xb\rangle=0$, the result is obvious. If $\langle\btheta_0^*-\btheta_{1}^*, \xb\rangle\neq0$, without loss of generality, we assume that $\btheta_0^*-\btheta_{1}^*>0$. Then the result is a direct consequence of the lemma below.

\begin{lemma}\label{lem:1d-tv-ineq}
Let $\epsilon$ be a random variable with mean 0 and a continuous symmetric distribution around 0. For any $\mu\in \RR$, $\mu\neq 0$, let $P_\mu$ and $P_{-\mu}$ denote the distribution of $\mu+\epsilon$ and $-\mu+\epsilon$ respectively. Then for any mapping $f:\RR\rightarrow \RR$,
\begin{equation}\label{eq-1d-tv-ineq}
\PP_{X\sim P_\mu}(f(X)\neq \sign(\mu))+\PP_{X\sim P_{-\mu}}(f(X)\neq \sign(-\mu))\geq 1-\|P_\mu-P_{-\mu}\|_{TV},
\end{equation}
and the equality can be attained when $f(x) = \sign(x)$.
%consider two hypothesis: $X\mathrel{\overset{\makebox[0pt]{\mbox{\tiny d}}}{=}}\mu+\epsilon$ and $X\mathrel{\overset{\makebox[0pt]{\mbox{\tiny d}}}{=}}-\mu+\epsilon$
\end{lemma}

Lemma \ref{lem:1d-tv-ineq} can be proved using only basic properties of the TV distance, so the proof is omitted.

(ii) can be similarly proved by applying Lemma \ref{lem:1d-tv-ineq} with $X$ corresponding to $\langle\btheta_0^*-\btheta_1^*, \tilde\xb_t\rangle$.

\section{Analysis of the proposed estimator (\ref{eq:proposed-estimator})}\label{pf:thm:theta-estimation}

\subsection{Proof of Theorem \ref{thm:theta-estimation}}

We fix some $t\in[T]$, and control $\|\hat\btheta_{a}^{(t)}-\btheta_a^*\|_2$ for $a\in\{0, 1\}$. Towards this goal, we combine analysis of the two random terms $\hat\bSigma_{\tilde\xb, a}^{(t)}$ and $\hat\bSigma_{\tilde\xb, r, a}^{(t)}$ in the lemma below.
\begin{lemma}\label{lem:hat-Sigma-x-r}
Under the same assumptions of Theorem \ref{thm:theta-estimation}, there exists an absolute constant $C$ such that with probability at least $1-4/t^2$, both of the followings hold:
\begin{align}
\bigg\|\hat\bSigma_{\tilde\xb, a}^{(t)}-\frac{1}{t}\sum_{\tau\in[t]}\pi_{\tau}^{nd}(a)(\xb_\tau\xb_{\tau}^\top+\bSigma_{e, \tau})\bigg\|_2\leq C\max\left\{\frac{d+\log t}{q_tt}, \sqrt{\frac{d+\log t}{q_tt}}\right\},\label{eq:hat-Sigma-x}\\
\bigg\|\hat\bSigma_{\tilde\xb, r, a}^{(t)}-\bigg(\frac{1}{t}\sum_{\tau\in[t]}\pi_{\tau}^{nd}(a)\xb_\tau \xb_{\tau}^\top\bigg)\btheta^*_{a}\bigg\|_2\leq CR\max\left\{\frac{d+\log t}{q_tt}, \sqrt{\frac{d+\log t}{q_tt}}\right\}.\label{eq:hat-Sigma-x-r}
\end{align}
\end{lemma}
Proof of Lemma \ref{lem:hat-Sigma-x-r} is in Section \ref{pf:lem:hat-Sigma-x-r}.

Denote $\bDelta_1 =\hat\bSigma_{\tilde\xb, a}^{(t)}-\frac{1}{t}\sum_{\tau\in[t]}\pi_{\tau}^{nd}(a)(\xb_\tau\xb_{\tau}^\top+\bSigma_{e, \tau})$, $\bDelta_2 = \hat\bSigma_{\tilde\xb, r, a}^{(t)}-\bigg(\frac{1}{t}\sum_{\tau\in[t]}\pi_{\tau}^{nd}(a)\xb_\tau \xb_{\tau}^\top\bigg)\btheta^*_{a}$. Then
\begin{align*}
\hat\btheta_a^{(t)}&= \bigg(\hat\bSigma_{\tilde\xb, a}^{(t)} - 
\frac{1}{t}\sum_{\tau\in[t]}\pi^{nd}_\tau(a)\bSigma_{e, \tau}\bigg)^{-1}\cdot
\hat\bSigma_{\tilde\xb, r, a}^{(t)}\\
& = \bigg(\frac{1}{t}\sum_{\tau\in[t]}\pi^{nd}_\tau(a)\xb_\tau\xb_{\tau}^\top+\bDelta_1\bigg)^{-1}\cdot \left[\bigg(\frac{1}{t}\sum_{\tau\in[t]}\pi_{\tau}^{nd}(a)\xb_\tau \xb_{\tau}^\top\bigg)\btheta^*_{a}+\bDelta_2\right]\\
&= \btheta_a^* - \bJ_1 + \bJ_2,
\end{align*}
where 
\begin{align*}
\bJ_1:=\left[\frac{1}{t}\sum_{\tau\in[t]}\pi_{\tau}^{nd}(a)\xb_\tau\xb_{\tau}^\top+\bDelta_1\right]^{-1}\cdot\bDelta_1\btheta_a^*,\quad
\bJ_2:=\left[\frac{1}{t}\sum_{\tau\in[t]}\pi_{\tau}^{nd}(a)\xb_\tau\xb_{\tau}^\top+\bDelta_1\right]^{-1}\cdot\bDelta_2.
\end{align*}
It's easy to verify that under the event where both (\ref{eq:hat-Sigma-x}) and (\ref{eq:hat-Sigma-x-r}) hold, whenever 
\begin{equation}\label{eq:condition-eigv-control}
C\max\left\{\frac{d+\log t}{q_tt}, \sqrt{\frac{d+\log t}{q_tt}}\right\}\leq \frac{\lambda_{0}}{2},
\end{equation}
we have 
$$
\|\bJ_1\|_2\leq \frac{2CR_{\btheta}}{\lambda_{0}}\max\left\{\frac{d+\log t}{q_tt}, \sqrt{\frac{d+\log t}{q_tt}}\right\}
$$
and 
$$
\|\bJ_2\|_2\leq \frac{2CR}{\lambda_{0}}\max\left\{\frac{d+\log t}{q_tt}, \sqrt{\frac{d+\log t}{q_tt}}\right\}.
$$
On the other hand, (\ref{eq:condition-eigv-control}) can be ensured by $t\geq \frac{C_1}{\min\{\lambda_{0}, \lambda_{0}^2\}}\frac{d+\log t}{q_t}$, where $C_1 = \max\{2C, 4C^2\}$. Given these guarantees, we have with probability at least $1-4/t^2$,
$$
\|\hat\btheta_a^{(t)}-\btheta_a^*\|_2\leq \|\bJ_1\|_2+\|\bJ_2\|_2\leq \frac{2C(R+R_{\btheta})}{\lambda_{0}}\max\left\{\frac{d+\log t}{q_tt}, \sqrt{\frac{d+\log t}{q_tt}}\right\}.
$$
Thus we conclude the proof.

\subsection{Additional comments on Assumption \ref{ass:min-signal}}

Following Remark \ref{rmk:ass:min-signal}, all the following examples of $\{\xb_\tau\}$ allow the existence of $\lambda_{0}$ with $\pi_\tau^{nd}(a)\equiv 1/2$ given any reasonably big $t$ with high probability:
\begin{itemize}
    \item $\{\xb_\tau\}$ is an i.i.d. sequence satisfying $\EE\xb_\tau\xb_\tau^\top\succeq \lambda_{1}I_d$, $\lambda_1>0$;
    \item $\{\xb_\tau\}$ is a weakly-dependent stationary time series (a common example is the multivariate ARMA process under regularity conditions, see e.g. \cite{banna2016bernstein}). The stationary distribution $P$ satisfies $\EE_{\xb\sim P}\xb\xb^\top\succeq \lambda_2I_d$, $\lambda_2>0$;
    \item $\{\xb_\tau\}$ is a periodic time series such that there exists $t_0\in \mathbb N^+$ which satisfies $\frac{1}{t_0}\sum_{\tau\in(kt_0+1, (k+1)t_0]}\xb_\tau\xb_\tau^\top\succeq \lambda_3I_d$ a.s. $\forall k\in\mathbb N$.
\end{itemize}

%\subsection{{Near optimality among policies with constant minimum sampling probability}}

%For fixed $p_0>0$, consider the data-independent policy $\{\pi_\tau\}_{\tau\geq 1}$ that always selects action 0 with probability $p_0$ and action 1 with probability $1-p_0$. Given this policy, $\cH_t = \{(\tilde\xb_\tau, A_\tau, Y_\tau)\}_{\tau\geq 1}$ consists of i.i.d. samples, where $A_\tau$ and $\tilde\xb_\tau$ are independent. Moreover, with high probability, the number of samples where $A_\tau = 0$ is $\cO(p_0t)$. Using results from classical statistics (e.g. \citep{van2000asymptotic}), among the reward model class $\{\btheta_0^*, \btheta_1^*\}\in \Theta$, the minimax lower bound $\ell_2$ error is of order $\Omega(\sqrt{\frac{d}{p_0t}})$. Combining Theorem 2.1, we see that the upper bound (2.7) is near-optimal among all policies with minimum sampling probability $p_0$ and $\{\btheta_0^*, \btheta_1^*\}\in \Theta$.

\subsection{{Generalization to off-policy method-of-moment estimation}}

(\ref{eq:proposed-estimator}) can be generalized to a class of method-of-moment estimators for off-policy learning. In this section, we delve into the general framework of off-policy method-of-moment estimation. This framework proves valuable in scenarios where a fully parametric model class for the reward is unavailable, yet there is a desire to estimate certain model parameters using offline batched bandit data.

For simplicity, we assume that $(X_t, Y_t(a):a\in\cA)_{t\in[T]}$ are drawn i.i.d. from an unknown distribution $\cP$. At each time $t\in[T]$, the action $A_t$ is drawn from a policy $\pi_t(\cdot|X_t, \cH_{t-1})$, and the agent observes only $o_t = (X_t, A_t, Y_t(A_t))$ together with the action selection probabilities $\pi_t$. Define the history up to time $t$ as $\cH_t = \{o_\tau\}_{\tau\leq t}$. For $a_0\in\cA$, we're interested in estimating $\btheta_{a_0}^*$, a $d$-dimensional parameter in $\cP^{(a_0)}$, which is the joint distribution of $\{X_t, Y_t(a_0)\}$. 

\begin{remark}
When the context is i.i.d., the problem of estimating $\{\btheta_a^*\}_{a\in\cA}$ in Section \ref{section2.3} is a special case of this setup by taking $\tilde\xb_t$ as $X_t$ and $r_t$ as $Y_t$.
\end{remark}

The traditional method-of-moment estimator looks for functions $f_1, \ldots, f_d$ as well as a mapping $\bphi:\RR^d\rightarrow \RR^d$, such that 
$$
\btheta_{a_0}^* = \bphi\big(\EE_{(X, Y)\sim \cP^{(a_0)}}f_1(X, Y), \ldots, \EE_{(X, Y)\sim \cP^{(a_0)}}f_d(X, Y)\big).
$$
Then, if given i.i.d. samples $(U_t, V_t)_{t\in[n]}$ from $\cP^{(a_0)}$, the estimator takes the form 
$$
\hat\btheta_{a_0} = \bphi\bigg(\frac{1}{T}\sum_{t\in[T]}f_1(U_t, V_t), \ldots, \frac{1}{T}\sum_{t\in[T]}f_d(U_t, V_t)\bigg).
$$
In fact, the naive estimator (\ref{eq:naive-estimator}) is of this form. It is clear that we cannot use this estimator for offline batched data $\cH_T$: There are no i.i.d. samples from $\cP^{(a_0)}$ because of the policy $\{\pi_t\}_{t\in[T]}$. Instead, we propose the following estimator: 
$$
\hat\btheta_{a_0} = \bphi\bigg(\frac{1}{T}\sum_{t\in[T]}W_tf_1(X_t, Y_t), \ldots, \frac{1}{T}\sum_{t\in[T]}W_tf_d(X_t, Y_t)\bigg),
$$
where $W_t = 1_{\{A_t = a_0\}}\frac{\pi^{nd}(A_t)}{\pi_t(A_t|X_t, \cH_{t-1})}$ for a data-independent probability distribution $\pi^{nd}$ on $\cA$. Similar to the proof of Theorem \ref{thm:theta-estimation}, it's not difficult to see that $\hat\btheta_{a_0}$ is consistent under mild conditions. In fact, (\ref{eq:proposed-estimator}) is a special case of this estimator when $\pi_{\tau}^{nd}$ does not depend on $\tau$. A more detailed analysis is left for future work.

\section{Analysis of \texttt{MEB}}\label{pf:cor:alg1-with-theta-estimation}

\subsection{Proof of Theorem \ref{thm-regret}}\label{pf:thm-regret}

At any time $t>T_0$, the instantaneous regret can be controlled by 
\begin{align}
{\text{Regret}}_t &= \EE_{a\sim \pi_t^\dagger}\langle \btheta^*_{a}, \tilde\xb_t\rangle - \EE_{a\sim \pi_t}\langle \btheta^*_{a}, \tilde\xb_t\rangle\nonumber\\
&=[(1-p_0)\langle\btheta^*_{a_t^\dagger}, \tilde\xb_t\rangle+p_0\langle\btheta^*_{1-a_t^\dagger}, \tilde\xb_t\rangle]-[(1-p_0)\langle\btheta^*_{\tilde a_t}, \tilde\xb_t\rangle+p_0\langle\btheta^*_{1-\tilde a_t}, \tilde\xb_t\rangle]\nonumber\\
&\leq (1-2p_0)1_{\{a_t^\dagger\neq \tilde a_t\}}\left|\langle \btheta^*_{a_t^\dagger} - \btheta^*_{1-a_t^\dagger}, \tilde\xb_t\rangle\right|.\label{eq:instant-regret}
\end{align}
Here recall that $a_t^\dagger:=\argmax_a\langle \btheta^*_{a}, \tilde\xb_t\rangle$, $\tilde a_t := \argmax_{a\in\{0, 1\}}\langle\hat\btheta_{a}^{(t-1)}, \tilde\xb_t\rangle$.

Note that $a_t^\dagger\neq \tilde a_t$ implies that 
\begin{align*}
\begin{cases}
\langle\btheta_{a_t^\dagger}^*, \tilde\xb_t\rangle\geq \langle\btheta_{1-a_t^\dagger}^*, \tilde\xb_t\rangle\\
\langle\hat\btheta_{a_t^\dagger}^{(t-1)}, \tilde\xb_t\rangle\leq \langle\hat\btheta_{1-a_t^\dagger}^{(t-1)}, \tilde\xb_t\rangle
\end{cases}
\end{align*}
which leads to 
\begin{align*}
\langle \btheta_{a_t^\dagger}^*, \tilde\xb_t\rangle&\geq \langle\btheta_{1-a_t^\dagger}^*, \tilde\xb_t\rangle\geq \langle\hat\btheta_{1-a_t^\dagger}^{(t-1)}, \tilde\xb_t\rangle - \max_a\|\hat\btheta_a^{(t-1)}-\btheta_a^*\|_2\\
&\geq \langle\hat\btheta_{a_t^\dagger}^{(t-1)}, \tilde\xb_t\rangle - \max_a\|\hat\btheta_a^{(t-1)}-\btheta_a^*\|_2\geq \langle\btheta_{a_t^\dagger}^*, \tilde\xb_t\rangle - 2\max_a\|\hat\btheta_a^{(t-1)}-\btheta_a^*\|_2,
\end{align*}
and further implies $\left|\langle \btheta^*_{a_t^\dagger} - \btheta^*_{1-a_t^\dagger}, \tilde\xb_t\rangle\right|\leq 2\max_a\|\hat\btheta_a^{(t-1)}-\btheta_a^*\|_2$.

Plugging in the above to (\ref{eq:instant-regret}) leads to an upper bound of instantaneous regret
$$
\text{Regret}_t\leq 2(1-2p_0)\max_a\|\hat\btheta_a^{(t-1)}-\btheta_a^*\|_2
$$
for $t>T_0$. We conclude the proof by summing up all instantaneous regret, and noticing that $\text{Regret}_t\leq 2R_\theta$ for any $t\leq T_0$.

\subsection{Proof of Corollary \ref{cor:alg1-with-theta-estimation}}\label{Appendix:subsection:Proof-of-corollary-2.1}

Under the assumptions of the Corollary, we first apply a union bound to Theorem \ref{thm:theta-estimation} to obtain that with probability at least $1-8/\sqrt{T}$, for all $t\geq \max\{\sqrt{T}, \frac{C_1}{\min\{\lambda_{0}, \lambda_{0}^2\}}\frac{d+\log t}{p_0}\}$, for all $a\in\{0, 1\}$,
\begin{equation}\label{eq:thm:theta-estimation-union}
    \|\hat\btheta_a^{(t)}-\btheta_a^*\|_2\leq \frac{C(R+R_{\btheta})}{\lambda_{0}}\max\left\{\frac{d+\log t}{p_{0}t}, \sqrt{\frac{d+\log t}{p_{0}t}}\right\}.
\end{equation}

Meanwhile, it's easy to verify that as long as $T\geq \max\{10, \frac{C'[d+\log(\sqrt{T})]^2}{\min\{\lambda_{0}^2, \lambda_{0}^4\}p_0^2}\}$ with $C'=C_1^2$ as in Theorem \ref{thm:theta-estimation}, $\forall t\geq \sqrt{T}$, $t\geq \frac{C_1}{\min\{\lambda_{0}, \lambda_{0}^2\}}\frac{d+\log t}{p_0}$. This implies that $\forall t>T_0$, $t/2\geq\max\{\sqrt{T}, \frac{C_1}{\min\{\lambda_{0}, \lambda_{0}^2\}}\frac{d+\log t}{p_0}\}$. Combining the results in Theorems \ref{thm:theta-estimation} and \ref{thm-regret}, we obtain that the regret of Algorithm \ref{alg1}
\begin{align*}
\text{Regret}(T)&\leq 4R_\theta\lceil\sqrt{T}\rceil + 2(1-2p_0)\sum_{t>T_0}\frac{C(R+R_\theta)}{\lambda_{0}} \max\left\{\frac{d+\log (t-1)}{p_0(t-1)}, \sqrt{\frac{d+\log (t-1)}{p_0(t-1)}}\right\}\\
&\leq 6R_\theta\sqrt{T} + \frac{2C(1-2p_0)(R+R_\theta)}{\lambda_{0}}\sum_{t>2\sqrt{T}} \max\left\{\frac{d+\log (\frac{1}{2} t)}{p_0\cdot\frac{1}{2} t}, \sqrt{\frac{d+\log (\frac{1}{2} t)}{p_0\cdot\frac{1}{2} t}}\right\}%\\
%&\leq \frac{2}{\alpha}R_\theta\sqrt{T} + \frac{2C(1-p_0)(R+R_\theta)}{\lambda_{\min}}\sum_{t>\sqrt{T}/\alpha} \max\left\{\frac{d+\log (\alpha t)}{p_0\alpha t}, \sqrt{\frac{d+\log (\alpha t)}{p_0\alpha t}}\right\}
\end{align*}
Here we use the fact that the mapping $u\mapsto \frac{d+\log u}{u}$ is monotonically decreasing on $[3,+\infty)$, and that $t-1\geq t/2\geq 3$ for all $t>2\sqrt{T}$ due to the assumptions of Corollary \ref{cor:alg1-with-theta-estimation}. Moreover, one can also verify that as long as $T\geq \max\{10, \frac{[d+\log(\sqrt{T})]^2}{p_0^2}\}$, we have $\forall t>2\sqrt{T}$, $\frac{d+\log (\frac{1}{2} t))}{p_0\cdot\frac{1}{2} t}\leq 1$. Thus, we can further deduce that
\begin{align}
\text{Regret}(T)
&\leq 6R_\theta\sqrt{T} + \frac{2C(1-2p_0)(R+R_\theta)}{\lambda_{0}}\sum_{t>2\sqrt{T}} \sqrt{\frac{d+\log (\frac12 t)}{p_0\cdot\frac12 t}}\nonumber\\
&\leq 6R_\theta\sqrt{T} + \frac{2\sqrt{2}C(1-2p_0)(R+R_\theta)}{\sqrt{p_0}\lambda_{0}}\left(\sqrt{d+\log \frac12 }\cdot \sum_{t>2\sqrt{T}} \sqrt{\frac{1}{t}}+\sum_{t>2\sqrt{T}} \sqrt{\frac{\log t}{t}}\right).\label{eq:regret-analysis-w-estimation}
\end{align}
Meanwhile, we have 
\begin{align}\label{eq-integral-analysis1}
\sum_{t>2\sqrt{T}} \sqrt{\frac{\log t}{t}}\leq 2\sum_{t=\lfloor2\sqrt{T}\rfloor+1}^T \frac{1}{2}\frac{\log t+1}{\sqrt{t\log t}}\leq 2\int_{\lfloor2\sqrt{T}\rfloor}^T\left(\frac{\mathrm d}{\mathrm d t}\sqrt{t\log t}\right)\mathrm d t\leq 2\sqrt{T\log T}.
\end{align}
Similarly one can obtain 
\begin{equation}\label{eq-integral-analysis2}
\sum_{t>2\sqrt{T}} \sqrt{\frac{1}{t}}\leq 2\sqrt{T}.
\end{equation}
Plug (\ref{eq-integral-analysis1}) and (\ref{eq-integral-analysis2}) into (\ref{eq:regret-analysis-w-estimation}), we deduce that
\begin{align*}
\text{Regret}(T)
&\leq 6R_\theta\sqrt{T} + \frac{2\sqrt{2}C(1-2p_0)(R+R_\theta)}{\sqrt{p_0}\lambda_{0}}\left(\sqrt{d-\log 2 }\cdot2\sqrt{T}+2\sqrt{T\log T}\right)\\
&\leq 6R_\theta\sqrt{T} + \frac{4\sqrt{2}C(1-2p_0)(R+R_\theta)}{\sqrt{p_0}\lambda_{0}}\sqrt{T}\left(\sqrt{d-\log 2}+\sqrt{\log T}\right),
\end{align*}
from which we conclude the proof.

\subsection{\texttt{MEB} with infrequent model update}
\begin{algorithm}[t]
\caption{\texttt{MEB} with infrequent model update}	
\label{alg2}
\begin{algorithmic}[1]		
\STATE \textbf{{Input}}: $\{\bSigma_{e, t}\}_{t\in[T]}$: covariance sequence of $\{\bepsilon_t\}_t$; $\{p_0^{(t)}\}_{t\in[T]}$: minimum selection probability at each time $t$; $\cS\subset [T]$: set of time points to update model estimates
\STATE $\hat\btheta_a \leftarrow 0$, $\forall a\in\{0, 1\}$  \thickspace \thickspace {\color{blue}$\%$\thinspace$\hat\btheta_a$ stores the most recent updated estimate of $\btheta_a^*$, only update if $t\in\cS$}
        \FOR{time $t = 1, 2, \ldots, T$}
        \IF{$\min_{s\in\cS}s\geq t$}
        \STATE Sample $a_t\sim \pi_t(\cdot|\tilde\xb_t, \cH_{t-1})$, where $\pi_t(a|\tilde\xb_t, \cH_{t-1}) = 1/2$ for all $a\in\{0, 1\}$\\
        {\color{blue} $\%$ If the model has never been learned before, explore with equal probability}
        \STATE \textbf{continue}
        \ENDIF
        \STATE $\tilde a_t \leftarrow \argmax_{a\in\{0, 1\}}\langle\hat\btheta_{a}, \tilde\xb_t\rangle$
        \STATE Sample $a_t\sim \pi_t(\cdot|\tilde\xb_t, \cH_{t-1})$, where $\pi_t(a|\tilde\xb_t, \cH_{t-1}):=
        \begin{cases}
        1-p_{0}^{(t)}, \quad\text{if }a = \tilde a_t\\
        p_{0}^{(t)}, \quad\text{otherwise}
        \end{cases}
        $
        \IF{$t\in\cS$}
        \STATE $\hat\btheta_a\leftarrow \hat\btheta_a^{(t)}$ as in (2.6)
        \ENDIF
        \ENDFOR
	\end{algorithmic}
\end{algorithm}

As mentioned at the end of Section \ref{section:meb}, in certain scenarios (e.g. when $d$ is large), we can save computational resources by updating the estimates of $(\btheta_a^*)_{a\in\{0, 1\}}$ less frequently. In Algorithm \ref{alg2}, we propose a variant of Algorithm \ref{alg1}. At each time $t$, given the noisy context $\tilde\xb_t$, the algorithm computes the best action $\tilde a_t$ according to the most recently updated estimators of $(\btheta_a^*)_{a\in\{0, 1\}}$. Then, it samples $\tilde a_t$ with probability $1-p_0^{(t)}$ and keeps an exploration probability of $p_0^{(t)}$ to sample the other action. In the meantime, the agent only has to update the estimate of $(\btheta_a^*)_{a\in\{0, 1\}}$ once in a while to save computation power: The algorithm specifies a subset $\cS\subset[T]$ and updates the estimators according to (\ref{eq:proposed-estimator}) only when $t\in\cS$. 

Under mild conditions, Algorithm \ref{alg2} achieves the same order of regret upper bound as Algorithm \ref{alg1}, as seen from Theorem \ref{thm-regret-S} and Corollary \ref{cor:alg1-with-theta-estimation-S} below. They are modified versions of Theorem \ref{thm-regret} and Corollary \ref{cor:alg1-with-theta-estimation}.

\begin{theorem}\label{thm-regret-S}
Let $s_{\min}:=\min_{s\in\cS}s$ be the first time Algorithm \ref{alg2} updates the model. Given Assumption \ref{ass:boundedness}, $\forall T_0\geq s_{\min}$, the regret of Algorithm \ref{alg2}
$$
\text{Regret}(T; \pi^\dagger)\leq 2T_0R_{\theta}+2(1-2p_0)\sum\nolimits_{t\in(T_0, T]}\max_{a\in\{0, 1\}}\|\hat\btheta_a^{(s_t)}-\btheta_a^*\|_2.
$$
Here for any $t\in[T]$, $s_t := \max\{s\in\cS: s<t\}$.
\end{theorem}

\begin{corollary}\label{cor:alg1-with-theta-estimation-S}
There exist constants $C, C'$ such that as long as the set of model update times $\cS$ satisfies: (i) $s_{\min}\leq \sqrt{T}$; (ii) $\forall t\in(\sqrt{T}, T]$, $s_t = \max\{s\in\cS: s<t\} \geq \alpha t$ for some constant $\alpha\in(e^{-d}, 1)$, then for any $T$ s.t. $T\geq C'\max\{1, \frac{d^2+\log^2({T})}{p_0^2}, \frac{d^2+\log^2({T})}{\min\{\lambda_{0}^2, \lambda_{0}^4\}p_0^2}\}$, with probability at least $1-\frac{16}{\sqrt{T}}$, the regret of Algorithm \ref{alg2}: $\text{Regret}(T; \pi^\dagger)\leq \frac{2R_\theta}{\alpha}\sqrt{T}+\frac{C(1-2p_0)(R+R_\theta)}{\lambda_{0}\sqrt{\alpha p_0}}\sqrt{T({d}+{\log T})}$.
\end{corollary}

Condition (i) and (ii) essentially requires Algorithm \ref{alg2} not to start learning the model too late, and to keep updating the learned model at least at time points with a `geometric' growth rate. This covers a wide range of choices of $\cS$ in practice. Two typical examples of $\cS$ could be: (1) $\cS=\{t\in[T]: t=kt_0\text{ for some }k\in\mathbb N^+\}$ (the model is learned every $t_0$ time points routinely, where $t_0$ is a constant integer); (2) If $1/\alpha\in \mathbb N^+$, $\cS=\{t\in[T]: t=(1/\alpha)^k\text{ for some }k\in\mathbb N^+\}$ (the model only needs to be learned $\cO(\log T)$ times to save computation).

The proof of Theorem \ref{thm-regret-S} is very similar to that of Theorem \ref{thm-regret}, and is thus omitted. The proof of Corollary \ref{cor:alg1-with-theta-estimation-S} is only slightly different from Corollary \ref{cor:alg1-with-theta-estimation}. For completeness, we briefly list the proof in Appendix \ref{pf:cor:alg1-with-theta-estimation-S}.

\section{Analysis with estimated error variance}\label{appendix:estimated-error-variance}

\subsection{{Proof of Theorem \ref{thm:theta-estimation-estimated-Sigma}}}

Fix $t\in[T]$ such that the conditions of Theorem \ref{thm:theta-estimation-estimated-Sigma} hold. Fix $a\in\{0, 1\}$. As in Appendix \ref{pf:thm:theta-estimation}, define $\bDelta_1 :=\hat\bSigma_{\tilde\xb, a}^{(t)}-\frac{1}{t}\sum_{\tau\in[t]}\pi_{\tau}^{nd}(a)(\xb_\tau\xb_{\tau}^\top+\bSigma_{e, \tau})$, $\bDelta_2 := \hat\bSigma_{\tilde\xb, r, a}^{(t)}-\bigg(\frac{1}{t}\sum_{\tau\in[t]}\pi_{\tau}^{nd}(a)\xb_\tau \xb_{\tau}^\top\bigg)\btheta^*_{a}$. We also let $\bDelta_3 := -\bDelta_t(a) = -\frac{1}{t}\sum_{\tau\in[t]}\pi_{\tau}^{nd}(a)(\hat\bSigma_{e, \tau} - \bSigma_{e, \tau})$. Recall Lemma \ref{lem:hat-Sigma-x-r}: with probability at least $1-4/t^2$, 
$$
\|\bDelta_1\|_2\leq C\max\left\{\frac{d+\log t}{q_tt}, \sqrt{\frac{d+\log t}{q_tt}}\right\},\quad \|\bDelta_2\|_2\leq CR\max\left\{\frac{d+\log t}{q_tt}, \sqrt{\frac{d+\log t}{q_tt}}\right\}.
$$
Meanwhile, 
\begin{align*}
\tilde\btheta_a^{(t)}&= \bigg(\hat\bSigma_{\tilde\xb, a}^{(t)} - 
\frac{1}{t}\sum_{\tau\in[t]}\pi^{nd}_\tau(a)\hat\bSigma_{e, \tau}\bigg)^{-1}\cdot
\hat\bSigma_{\tilde\xb, r, a}^{(t)}\\
& = \bigg(\frac{1}{t}\sum_{\tau\in[t]}\pi^{nd}_\tau(a)\xb_\tau\xb_{\tau}^\top+\bDelta_1+\bDelta_3\bigg)^{-1}\cdot \left[\bigg(\frac{1}{t}\sum_{\tau\in[t]}\pi_{\tau}^{nd}(a)\xb_\tau \xb_{\tau}^\top\bigg)\btheta^*_{a}+\bDelta_2\right]\\
&= \btheta_a^* - \bJ_1' + \bJ_2',
\end{align*}
where 
\begin{align*}
\bJ_1':=\bigg[\frac{1}{t}\sum_{\tau\in[t]}\pi_{\tau}^{nd}(a)\xb_\tau\xb_{\tau}^\top+\bDelta_1+\bDelta_3\bigg]^{-1}(\bDelta_1+\bDelta_3)\btheta_a^*,\thickspace
\bJ_2':=\bigg[\frac{1}{t}\sum_{\tau\in[t]}\pi_{\tau}^{nd}(a)\xb_\tau\xb_{\tau}^\top+\bDelta_1+\bDelta_3\bigg]^{-1}\bDelta_2.
\end{align*}
Under the events where both (\ref{eq:hat-Sigma-x}) and (\ref{eq:hat-Sigma-x-r}) hold, whenever 
\begin{equation}\label{eq:condition-eigv-control-estimated-Sigma}
C\max\left\{\frac{d+\log t}{q_tt}, \sqrt{\frac{d+\log t}{q_tt}}\right\}\leq \frac{\lambda_{0}}{4}
\end{equation}
and $\|\bDelta_3\|_2\leq \frac{\lambda_{0}}{4}$, we have 
$$
\|\bJ_1'\|\leq \frac{2R_{\btheta}}{\lambda_{0}}\left(C\max\left\{\frac{d+\log t}{q_tt}, \sqrt{\frac{d+\log t}{q_tt}}\right\} + \|\bDelta_3\|_2\right)
$$
and 
$$
\|\bJ_2'\|\leq \frac{2CR}{\lambda_{0}}\max\left\{\frac{d+\log t}{q_tt}, \sqrt{\frac{d+\log t}{q_tt}}\right\}.
$$
On the other hand, (\ref{eq:condition-eigv-control-estimated-Sigma}) can be ensured by $t\geq \frac{C_1'}{\min\{\lambda_{0}, \lambda_{0}^2\}}\frac{d+\log t}{q_t}$, where $C_1' = \max\{4C, 16C^2\}$. Given these guarantees, we have with probability at least $1-4/t^2$, 
$$
\|\tilde\btheta_a^{(t)}-\btheta_a^*\|\leq \|\bJ_1'\|_2+\|\bJ_2'\|_2\leq \frac{2C(R+R_{\btheta})}{\lambda_{0}}\max\left\{\frac{d+\log t}{q_tt}, \sqrt{\frac{d+\log t}{q_tt}}\right\} + \frac{2R_\theta}{\lambda_0}\|\bDelta_t(a)\|_2.
$$
Thus we conclude the proof.

\subsection{{Proof of Corollary \ref{cor:alg1-with-theta-estimation-estimated-Sigma}}}

As in Appendix \ref{Appendix:subsection:Proof-of-corollary-2.1}, we first apply a union bound to Theorem \ref{thm:theta-estimation-estimated-Sigma} to obtain that with probability at least $1-8/\sqrt{T}$, for all $t\geq \max\{\sqrt{T}, \frac{C_1'}{\min\{\lambda_{0}, \lambda_{0}^2\}}\frac{d+\log t}{p_0}\}$, for all $a\in\{0, 1\}$,
\begin{equation}\label{eq:thm:theta-estimation-union-estimated-Sigma}
    \|\tilde\btheta_a^{(t)}-\btheta_a^*\|_2\leq \frac{C(R+R_{\btheta})}{\lambda_{0}}\max\left\{\frac{d+\log t}{p_{0}t}, \sqrt{\frac{d+\log t}{p_{0}t}}\right\} + \frac{2R_\theta}{\lambda_0}\|\bDelta_t(a)\|_2.
\end{equation}
Meanwhile, it's easy to verify that as long as $T\geq \max\{10, \frac{C''[d+\log(\sqrt{T})]^2}{\min\{\lambda_{0}^2, \lambda_{0}^4\}p_0^2}\}$ with $C''=C_1'^2$ as in Theorem \ref{thm:theta-estimation-estimated-Sigma}, $\forall t\geq \sqrt{T}$, $t\geq \frac{C_1'}{\min\{\lambda_{0}, \lambda_{0}^2\}}\frac{d+\log t}{p_0}$. This implies that $\forall t>T_0$, $t/2\geq\max\{\sqrt{T}, \frac{C_1'}{\min\{\lambda_{0}, \lambda_{0}^2\}}\frac{d+\log t}{p_0}\}$. Combining the results in Theorems \ref{thm-regret} and \ref{thm:theta-estimation-estimated-Sigma}, we obtain that the regret of Algorithm \ref{alg1} with $(\tilde\btheta_a^{(t)})_{a\in\{0, 1\}, t\in[T]}$ as plugin estimators:
\begin{align*}
\text{Regret}(T)&\leq 4R_\theta\lceil\sqrt{T}\rceil + 2(1-2p_0)\sum_{t>T_0}\bigg[\frac{C(R+R_\theta)}{\lambda_{0}} \max\bigg\{\frac{d+\log (t-1)}{p_0(t-1)}, \sqrt{\frac{d+\log (t-1)}{p_0(t-1)}}\bigg\}\\
& \quad + \frac{2R_\theta}{\lambda_0}\max_{a\in\{0, 1\}}\|\bDelta_{t-1}(a)\|_2\bigg].
\end{align*}
We use the same arguments as in Appendix \ref{Appendix:subsection:Proof-of-corollary-2.1} to upper bound the first part of the right-hand side:
\begin{align*}
&4R_\theta\lceil\sqrt{T}\rceil + 2(1-2p_0)\sum_{t>T_0}\frac{C(R+R_\theta)}{\lambda_{0}} \max\bigg\{\frac{d+\log (t-1)}{p_0(t-1)}, \sqrt{\frac{d+\log (t-1)}{p_0(t-1)}}\bigg\}\\
\leq & 6R_\theta\sqrt{T} + \frac{4\sqrt{2}C(1-2p_0)(R+R_\theta)}{\sqrt{p_0}\lambda_{0}}\sqrt{T}\left(\sqrt{d-\log 2}+\sqrt{\log T}\right)
\end{align*}
given $T$ satisfies the conditions of the corollary. The proof is concluded by plugging this into the regret upper bound above.

\section{Additional proofs}

\subsection{Proof of Theorem \ref{thm:regret-multiple-actions}}\label{pf:thm:regret-multiple-actions}
At any time $t>T_0$, the instantaneous regret can be controlled by 
\begin{align}
{\text{Regret}}_t &= \EE_{a\sim \pi_t^\dagger}\langle \btheta^*_{a}, \tilde\xb_t\rangle - \EE_{a\sim \pi_t}\langle \btheta^*_{a}, \tilde\xb_t\rangle\nonumber\\
&\leq (1-Kp_0)1_{\{a_t^\dagger\neq \tilde a_t\}}\left|\langle \btheta^*_{a_t^\dagger} - \btheta^*_{\tilde a_t}, \tilde\xb_t\rangle\right|.\label{eq:instant-regret-multiple-actions}
\end{align}
Here recall that $a_t^\dagger:=\argmax_a\langle \btheta^*_{a}, \tilde\xb_t\rangle$, $\tilde a_t := \argmax_{a\in\{0, 1\}}\langle\hat\btheta_{a}^{(t-1)}, \tilde\xb_t\rangle$.

Note that $a_t^\dagger\neq \tilde a_t$ implies that 
\begin{align*}
\begin{cases}
\langle\btheta_{a_t^\dagger}^*, \tilde\xb_t\rangle\geq \langle\btheta_{\tilde a_t}^*, \tilde\xb_t\rangle\\
\langle\hat\btheta_{a_t^\dagger}^{(t-1)}, \tilde\xb_t\rangle\leq \langle\hat\btheta_{\tilde a_t}^{(t-1)}, \tilde\xb_t\rangle
\end{cases}
\end{align*}
which leads to 
\begin{align*}
\langle \btheta_{a_t^\dagger}^*, \tilde\xb_t\rangle&\geq \langle\btheta_{\tilde a_t}^*, \tilde\xb_t\rangle\geq \langle\hat\btheta_{\tilde a_t}^{(t-1)}, \tilde\xb_t\rangle - \max_a\|\hat\btheta_a^{(t-1)}-\btheta_a^*\|_2\\
&\geq \langle\hat\btheta_{a_t^\dagger}^{(t-1)}, \tilde\xb_t\rangle - \max_a\|\hat\btheta_a^{(t-1)}-\btheta_a^*\|_2\geq \langle\btheta_{a_t^\dagger}^*, \tilde\xb_t\rangle - 2\max_a\|\hat\btheta_a^{(t-1)}-\btheta_a^*\|_2,
\end{align*}
and further implies $\left|\langle \btheta^*_{a_t^\dagger} - \btheta^*_{\tilde a_t}, \tilde\xb_t\rangle\right|\leq 2\max_a\|\hat\btheta_a^{(t-1)}-\btheta_a^*\|_2$.

Plugging in the above to (\ref{eq:instant-regret-multiple-actions}) leads to an upper bound of instantaneous regret
$$
\text{Regret}_t\leq 2(1-Kp_0)\max_a\|\hat\btheta_a^{(t-1)}-\btheta_a^*\|_2
$$
for $t>T_0$. We conclude the proof by summing up all instantaneous regret, and noticing that $\text{Regret}_t\leq 2R_\theta$ for any $t\leq T_0$.

\subsection{Proof of Theorem \ref{thm:standard-benchmark-multiple-actions}}\label{pf:thm:standard-benchmark-multiple-actions}

As in the proof of Theorem \ref{thm:standard-benchmark}, we have $q_t = \min_{\tau\leq t, a\in\{0, 1\}}\pi_\tau(a|\tilde\xb_t, \cH_{\tau-1}) = p_0^{(t)}$. Theorem \ref{thm:theta-estimation} indicates that, as long as 
\begin{equation}\label{eq:standard-benchmark-multiple-actions-condition1}
p_0^{(t)}\geq \frac{C_1}{\lambda_0\wedge\lambda_0^2}\frac{d+\log t}{t},
\end{equation}
with probability at least $1-\frac{4K}{t^2}$, for any $a\in\{0, 1\}$
\begin{equation}\label{eq:standard-benchmark-multiple-actions-estimation-error}
\|\hat\btheta_a^{(t)}-\btheta_a^*\|_2
\leq \frac{C(R+R_\theta)}{\lambda_0}\max\left\{\frac{d+\log t}{t^{\frac23}}, \sqrt{\frac{d+\log t}{t^{\frac23}}}\right\}.
\end{equation}

At any time $t>T_0$, the instantaneous regret can be controlled by 
\begin{align}
{\text{Regret}}_t^* &= \EE_{a\sim \pi_t^*}\langle \btheta^*_{a}, \tilde\xb_t\rangle - \EE_{a\sim \pi_t}\langle \btheta^*_{a}, \tilde\xb_t\rangle\nonumber\\
&=\langle\btheta^*_{a_t^\dagger}, \tilde\xb_t\rangle-\big[(1-(K-1)p_0^{(t)})\langle\btheta^*_{\tilde a_t}, \tilde\xb_t\rangle+\sum_{a\neq \tilde a_t}p_0^{(t)}\langle\btheta^*_{a}, \tilde\xb_t\rangle\big]\nonumber\\
&= p_0^{(t)}\sum_{a\neq a_t^\dagger}\langle \btheta^*_{a_t^\dagger} - \btheta^*_{a}, \tilde\xb_t\rangle + 1_{\{a_t^\dagger\neq \tilde a_t\}}(1-Kp_0^{(t)})\langle \btheta^*_{a_t^\dagger} - \btheta^*_{\tilde a_t}, \tilde\xb_t\rangle\nonumber\\
&\leq 2(K-1)p_0^{(t)}R_\theta + 1_{\{a_t^\dagger\neq \tilde a_t\}}\langle \btheta^*_{a_t^\dagger} - \btheta^*_{\tilde a_t}, \tilde\xb_t\rangle.\label{eq:instant-regret-standard-benchmark-multiple-actions}
\end{align}
Here recall that $a_t^\dagger:=\argmax_a\langle \btheta^*_{a}, \tilde\xb_t\rangle$, $\tilde a_t := \argmax_{a\in\{0, 1\}}\langle\hat\btheta_{a}^{(t-1)}, \tilde\xb_t\rangle$.

Note that $a_t^\dagger\neq \tilde a_t$ implies that 
\begin{align*}
\begin{cases}
\langle\btheta_{a_t^\dagger}^*, \tilde\xb_t\rangle\geq \langle\btheta_{\tilde a_t}^*, \tilde\xb_t\rangle\\
\langle\hat\btheta_{a_t^\dagger}^{(t-1)}, \tilde\xb_t\rangle\leq \langle\hat\btheta_{\tilde a_t}^{(t-1)}, \tilde\xb_t\rangle
\end{cases}
\end{align*}
which leads to 
\begin{align*}
\langle \btheta_{a_t^\dagger}^*, \tilde\xb_t\rangle&\geq \langle\btheta_{\tilde a_t}^*, \tilde\xb_t\rangle\geq \langle\hat\btheta_{\tilde a_t}^{(t-1)}, \tilde\xb_t\rangle - \max_a\|\hat\btheta_a^{(t-1)}-\btheta_a^*\|_2\\
&\geq \langle\hat\btheta_{a_t^\dagger}^{(t-1)}, \tilde\xb_t\rangle - \max_a\|\hat\btheta_a^{(t-1)}-\btheta_a^*\|_2\geq \langle\btheta_{a_t^\dagger}^*, \tilde\xb_t\rangle - 2\max_a\|\hat\btheta_a^{(t-1)}-\btheta_a^*\|_2,
\end{align*}
and further implies $\left|\langle \btheta^*_{a_t^\dagger} - \btheta^*_{\tilde a_t}, \tilde\xb_t\rangle\right|\leq 2\max_a\|\hat\btheta_a^{(t-1)}-\btheta_a^*\|_2$.

Plugging in the above to (\ref{eq:instant-regret-standard-benchmark-multiple-actions}) leads to an upper bound of instantaneous regret
\begin{align*}
\text{Regret}_t^*&\leq 2(K-1)p_0^{(t)}R_\theta + 2\max_a\|\hat\btheta_a^{(t-1)}-\btheta_a^*\|_2 \\
&\leq \frac{2(K-1)R_\theta}{t^{\frac13}} + 
\frac{2C(R+R_\theta)}{\lambda_0}\max\left\{\frac{d+\log (t-1)}{(t-1)^{\frac23}}, \sqrt{\frac{d+\log (t-1)}{(t-1)^{\frac23}}}\right\}\\
&\leq \frac{2(K-1)R_\theta}{t^{\frac13}} + \frac{2C(R+R_\theta)}{\lambda_0}\max\left\{\frac{d+\log t}{(t/2)^{\frac23}}, \sqrt{\frac{d+\log t}{(t/2)^{\frac23}}}\right\}\\
&\leq \frac{2(K-1)R_\theta}{t^{\frac13}} + \frac{4C(R+R_\theta)}{\lambda_0}\max\left\{\frac{d+\log t}{t^{\frac23}}, \sqrt{\frac{d+\log t}{t^{\frac23}}}\right\}
\end{align*}
for $t>T_0$. If in addition, for all $t\geq T_0$,
\begin{equation}\label{eq:standard-benchmark-multiple-actions-condition2}
\frac{d+\log t}{t^{\frac23}}\leq 1,
\end{equation}
then we further have
\begin{align*}
\text{Regret}_t^*
&\leq \frac{2(K-1)R_\theta}{t^{\frac13}} + \frac{4C(R+R_\theta)}{\lambda_0}\sqrt{\frac{d+\log t}{t^{\frac23}}}
\end{align*}
for $t>T_0$. Meanwhile, notice that $\text{Regret}_t^*\leq 2R_\theta$ for any $t\leq T_0$. Thus, we deduce that the cumulative regret compared to the standard benchmark:
\begin{align}
\text{Regret}(T;\pi^*)
&\leq T_0\cdot 2R_\theta + \sum_{t>2T^{\frac23}}\left(2(K-1)R_\theta t^{-\frac13}+\frac{4C(R+R_\theta)}{\lambda_0}t^{-\frac13}\sqrt{d+\log t}\right)\nonumber\\
&\leq C_2\left\{(K-1)R_\theta T^{\frac23} + \frac{R+R_\theta}{\lambda_0}T^{\frac23}\sqrt{d+\log T}\right\}
\end{align}
For a universal constant $C_2$. Finally, conditions (\ref{eq:standard-benchmark-multiple-actions-condition1}) and (\ref{eq:standard-benchmark-multiple-actions-condition2}) can be guaranteed by $T\geq C_3\max\{1, (d+\log T)^{\frac94}, \big(\frac{d+\log T}{\lambda_0\wedge\lambda_0^2}\big)^{\frac94}\}$ for some universal constant $C_3$.

\subsection{Proof of Lemma \ref{lem:hat-Sigma-x-r}}\label{pf:lem:hat-Sigma-x-r}
We first analyze $\hat\bSigma_{\tilde\xb, a}^{(t)}$. Notice that $\hat\bSigma_{\tilde\xb, a}^{(t)}=\frac{1}{t}\sum_{\tau\in[t]}\bV_{\tau, a}$, where $\bV_{\tau, a}=\frac{\pi_{\tau}^{nd}(A_t)}{\pi_\tau(A_t|\tilde\xb_t, \cH_{t-1})}1_{\{A_t=a\}}\tilde\xb_\tau\tilde\xb_{\tau}^\top$.  For any fixed $\bu\in\mathbb S^{d-1}:= \{\bu'\in \mathbb R^d: \|\bu'\|_2=1\}$, $(v_{\bu, \tau, a}:=\bu^\tau[\bV_{\tau, a}-\EE[\bV_{\tau, a}|\cH_{\tau-1}]]\bu)_\tau$ is a martingale difference sequence. Moreover, it's easy to verify that $|v_{\bu, \tau, a}|\leq \frac{2}{q_t}$ and
\begin{align*}
    \Var(v_{\bu, \tau, a}|\cH_{\tau-1})&
    \leq \EE[(\bu^\top \bV_{\tau, a}\bu)^2|\cH_{\tau-1}]=\EE\left[\left(\frac{\pi_{\tau}^{nd}(A_\tau)}{\pi_\tau(A_\tau|\tilde\xb_\tau, \cH_{\tau-1})}\right)^21_{\{A_\tau=a\}}(\bu^\top\tilde\xb\tilde\xb^\top\bu)^2\bigg|\cH_{\tau-1}\right]\\
    &=\EE_{\bepsilon_\tau, A_\tau\sim \pi_{\tau}^{nd}(\cdot)}\left[\left(\frac{\pi_{\tau}^{nd}(A_\tau)}{\pi_\tau(A_\tau|\tilde\xb_\tau, \cH_{\tau-1})}\right)1_{\{A_\tau=a\}}(\bu^\top\tilde\xb\tilde\xb^\top\bu)^2\bigg|\cH_{\tau-1}\right]\leq \frac{1}{q_t}.
\end{align*}

According to Freedman's Inequality \citep{freedman1975tail}, for any $\gamma_1, \gamma_2>0$, 
$$
\PP\left(\sum_{\tau\in[t]}v_{\bu, \tau, a}\geq \gamma_1, \sum_{\tau\in[t]}\Var(v_{\bu, \tau, a}|\cH_{\tau-1})\leq \gamma_2\right)\leq e^{-\frac{\gamma_1^2}{2(\frac{2}{q_t}\gamma_1+\gamma_2)}}.
$$
Set $\gamma_2 = t/q_t$, and we obtain 
$\PP\left(\sum_{\tau\in[t]}v_{\bu, \tau, a}\geq \gamma_1\right)\leq e^{-\frac{q_t\gamma_1^2}{2(2\gamma_1+t)}}
$. Applying the same analysis to $(-v_{\bu, \tau, a})_\tau$ and combining the results gives $\PP\left(|\sum_{\tau\in[t]}v_{\bu, \tau, a}|\geq \gamma_1\right)\leq 2e^{-\frac{q_t\gamma_1^2}{2(2\gamma_1+t)}}
$.

Denote $\bM_t= \frac{1}{t}\sum_{\tau\in[t]}(\bV_{\tau, a}-\EE[\bV_{\tau, a}|\cH_{\tau-1}])$, then the above means that $\forall \bu\in\mathbb S^{d-1}$, 
\begin{equation}\label{eq:v-concentration-singledirection} 
  \PP\left(|\bu^\top\bM_t\bu|\geq \frac{\gamma_1}{t}\right)\leq 2e^{-\frac{q_t\gamma_1^2}{2(2\gamma_1+t)}}.
\end{equation}%
Let $\cN$ be a $\frac{1}{4}$-net of $\mathbb S^{d-1}$, $|\cN|\leq 9^d$. $\forall \bu\in\mathbb S^{d-1}$, find $\bu'\in\cN$ s.t. $\|\bu-\bu'\|_2\leq \frac{1}{4}$, and we have 
$$
|\bu^\top \bM_t\bu-\bu'^\top\bM_t\bu'|\leq |\bu^\top \bM_t(\bu-\bu')| + |\bu'^\top\bM_t(\bu-\bu')|\leq \frac12 \|\bM_t\|_2.
$$
This implies that 
$$
\|\bM_t\|_2 = \sup_{\bu\in\mathbb S^{d-1}}|\bu^\top\bM_t\bu|\leq \sup_{\bu'\in\mathcal \cN}|\bu'^\top\bM_t\bu'|+\frac12 \|\bM_t\|_2,
$$
and thus $\sup_{\bu\in\cN}|\bu^\top\bM_t\bu|\geq\frac12\|\bM_t\|_2$.
Combining the above and (\ref{eq:v-concentration-singledirection}), we obtain that for any $\gamma_1>0$,
\begin{align*}
\PP\left(\|\bM_t\|_2\geq \frac{2\gamma_1}{t}\right)\leq \PP\left(\sup_{\bu\in\cN}|\bu^\top\bM_t\bu|\geq \frac{\gamma_1}{t}\right)\leq 9^d\cdot \PP\left(|\bu^\top\bM_t\bu|\geq \frac{\gamma_1}{t}\right)=2\cdot 9^d\cdot e^{-\frac{q_t\gamma_1^2}{2(2\gamma_1+t)}}.
\end{align*}
By choosing $\gamma_1 = 48\max\{\frac{d+\log t}{q_t}, \sqrt{\frac{d+\log t}{q_t}}\}$, and noticing that \\$\bM_t = \hat\bSigma_{\tilde\xb, a}^{(t)}-\frac{1}{t}\sum_{\tau\in[t]}\EE[\bV_{\tau, a}|\cH_{\tau-1}]$, we have
\begin{equation}\label{eq:hat-Sigma-x-1}
\PP\left(\bigg\|\hat\bSigma_{\tilde\xb, a}^{(t)}-\frac{1}{t}\sum_{\tau\in[t]}\EE[\bV_{\tau, a}|\cH_{\tau-1}]\bigg\|_2\geq 96\max\left\{\frac{d+\log t}{q_tt}, \sqrt{\frac{d+\log t}{q_tt}}\right\}\right)\leq \frac{2}{t^2}.
\end{equation}
On the other hand, we have 
\begin{align}
\EE[\bV_{\tau, a}|\cH_{\tau-1}]
&= \EE_{\bepsilon_\tau}\left[\EE_{A_\tau\sim\pi_\tau(\cdot|\tilde\xb_{\tau}, \cH_{\tau-1})}\bigg[\frac{\pi_{\tau}^{nd}(A_\tau)}{\pi_\tau(A_\tau|\tilde\xb_\tau, \cH_{\tau-1})}1_{\{A_\tau=a\}}\tilde\xb_\tau\tilde\xb_{\tau}^\top\big|\bepsilon_\tau, \cH_{\tau-1}\bigg]\bigg|\cH_{\tau-1}\right]\nonumber\\
& =\EE_{\bepsilon_\tau}\left[\EE_{A_\tau\sim\pi_{\tau}^{nd}(\cdot)}\big[1_{\{A_\tau=a\}}\tilde\xb_\tau\tilde\xb_{\tau}^\top\big|\bepsilon_\tau, \cH_{\tau-1}\big]\bigg|\cH_{\tau-1}\right]\nonumber\\
& =\EE_{\bepsilon_\tau}\left[\pi_{\tau}^{nd}(a)\cdot\tilde\xb_\tau\tilde\xb_{\tau}^\top\bigg|\cH_{\tau-1}\right]\nonumber\\
&=\pi_{\tau}^{nd}(a)(\xb_\tau\xb_{\tau}^\top+\bSigma_{e, \tau}).\label{eq:condition-e-V}
\end{align}
Here we've used the facts that (i) $\{\pi_{\tau}^{nd}\}_{\tau}$ is data-independent; (ii) $\EE[\bepsilon_\tau|\cH_{\tau-1}] = 0$, $\Var[\bepsilon_\tau|\cH_{\tau-1}] = \bSigma_{e, \tau}$.
Plug (\ref{eq:condition-e-V}) into (\ref{eq:hat-Sigma-x-1}), and we get
\begin{equation}\label{eq:hat-Sigma-x-2}
\PP\left(\bigg\|\hat\bSigma_{\tilde\xb, a}^{(t)}-\frac{1}{t}\sum_{\tau\in[t]}\pi_{\tau}^{nd}(a)(\xb_\tau\xb_{\tau}^\top+\bSigma_{e, \tau})\bigg\|_2\geq 96\max\left\{\frac{d+\log t}{q_tt}, \sqrt{\frac{d+\log t}{q_tt}}\right\}\right)\leq \frac{2}{t^2}.
\end{equation}

The analysis for $\hat\bSigma_{\tilde\xb, r, a}^{(t)}$ is similar. Write $\hat\bSigma_{\tilde\xb, r, a}^{(t)}=\frac{1}{t}\sum_{\tau\in[t]}\bZ_{\tau, a}$, $\bZ_{\tau, a}:=\frac{\pi_{\tau}^{nd}(A_t)}{\pi_\tau(A_\tau|\tilde\xb_\tau, \cH_{\tau-1})}1_{\{A_t = a\}}\tilde\xb_tr_t$. Then for any $\bu\in \mathcal S^{d-1}$, it's easy to verify that $|(\bZ_{\tau, a}-\EE[\bZ_{\tau, a}|\cH_{\tau-1}])^\top\bu|\leq \frac{2R}{q_t}$, and $\Var((\bZ_{\tau, a}-\EE[\bZ_{\tau, a}|\cH_{\tau-1}])^\top\bu)\leq \EE[(\bZ_{\tau, a}^\top\bu)^2|\cH_{\tau-1}]\leq\frac{R^2}{q_t}$. Applying Freedman's Inequality leads to 
\begin{equation}\label{eq:z-concentration-singledirection}
\PP\left(|\bw_t^\top \bu|\geq \frac{\gamma_1}{t}\right)\leq 2e^{-\frac{q_t\gamma_1^2}{2(2R\gamma_1+R^2t)}},
\end{equation}
where $\bw_t:=\frac{1}{t}\sum_{\tau\in[t]}(\bZ_{\tau, a}-\EE[\bZ_{\tau, a}|\cH_{\tau-1}])$. 

Recall that $\cN$ is a $\frac{1}{4}$-net of $\mathbb S^{d-1}$, $|\cN|\leq 9^d$. $\forall \bu\in\mathbb S^{d-1}$, find $\bu'\in\mathbb S^{d-1}$ s.t. $\|\bu-\bu'\|\leq 1/4$, then $|\bw_t^\top\bu-\bw_t^\top \bu'|\leq \frac{1}{4}\|\bw_t\|_2$, and thus 
$$
\|\bw_t\|_2=\sup_{\bu\in\mathbb S^{d-1}}|\bw_t^\top\bu|\leq \sup_{\bu'\in\cN}|\bw_t^\top\bu'|+\frac14 \|\bw_t\|_2
$$
which implies that $\sup_{\bu\in\cN}|\bw_t^\top \bu|\geq \frac34 \|\bw_t\|_2$. Taking this and (\ref{eq:z-concentration-singledirection}) into account, we derive that
$$
\PP\left(\|\bw_t\|_2\geq \frac{4}{3}\frac{\gamma_1}{t}\right)\leq \PP\left(\sup_{\bu\in\cN}|\bw_t^\top\bu|\geq \frac{\gamma_1}{t}\right)\leq 9^d\cdot 2e^{-\frac{q_t\gamma_1^2}{2(2R\gamma_1+R^2t)}}
$$
By choosing $\gamma_1=48R\max\left\{\frac{d+\log t}{t}, \sqrt{\frac{d+\log t}{t}}\right\}$ and noticing that $\bw_t = \hat\bSigma_{\tilde\xb, r, a}^{(t)}-\frac{1}{t}\sum_{\tau\in[t]}\EE[\bZ_{\tau, a}|\cH_{\tau-1}]$, we obtain that
\begin{equation}\label{eq:hat-Sigma-x-r-1}
\PP\left(\bigg\|\hat\bSigma_{\tilde\xb, r, a}^{(t)}-\frac{1}{t}\sum_{\tau\in[t]}\EE[\bZ_{\tau, a}|\cH_{\tau-1}]\bigg\|_2\geq 64R\max\left\{\frac{d+\log t}{q_tt}, \sqrt{\frac{d+\log t}{q_tt}}\right\}\right)\leq \frac{2}{t^2}.
\end{equation}
Finally, because 
\begin{align*}
\EE[\bZ_{\tau, a}|\cH_{\tau-1}]
&=\EE_{\bepsilon_\tau}\left[\EE_{A_\tau\sim\pi_\tau(\cdot|\tilde\xb_\tau, \cH_{\tau-1}), \eta_\tau}\left[\frac{\pi_{\tau}^{nd}(A_\tau)}{\pi_{\tau}(A_\tau|\tilde\xb_\tau, \cH_{\tau-1})}1_{\{A_\tau=a\}}\tilde\xb_\tau r_\tau\big|\cH_{\tau-1}, \bepsilon_\tau\right]\bigg|\cH_{\tau-1}\right]\\
&=\EE_{\bepsilon_\tau}\left[\EE_{A_\tau\sim\pi_{\tau}^{nd}(\cdot), \eta_\tau}\left[1_{\{A_\tau=a\}}\tilde\xb_\tau r_\tau|\cH_{\tau-1}, \bepsilon_\tau\right]\bigg|\cH_{\tau-1}\right]\\
&=\EE_{\bepsilon_\tau}\left[\EE_{A_\tau\sim\pi_{\tau}^{nd}(\cdot), \eta_\tau}\left[1_{\{A_\tau=a\}}\tilde\xb_\tau (\xb_{\tau}^\top\btheta^*_{a}+\eta_\tau)|\cH_{\tau-1}, \bepsilon_\tau\right]\bigg|\cH_{\tau-1}\right]\\
&=\EE_{\bepsilon_\tau}\left[\pi_{\tau}^{nd}(a)\EE_{\eta_\tau}\left[\tilde\xb_\tau (\xb_{\tau}^\top\btheta^*_{a}+\eta_\tau)|\cH_{\tau-1}, \bepsilon_\tau\right]\bigg|\cH_{\tau-1}\right]\\
&=\pi_{\tau}^{nd}(a)\EE_{\bepsilon_\tau}\left[\tilde\xb_\tau \xb_{\tau}^\top\btheta^*_{a}\bigg|\cH_{\tau-1}\right]=\pi_{\tau}^{nd}(a)(\xb_\tau \xb_{\tau}^\top)\btheta^*_{a},
\end{align*}
Plug in (\ref{eq:hat-Sigma-x-r-1}), and we obtain 
\begin{equation}\label{eq:hat-Sigma-x-r-2}
\PP\left(\bigg\|\hat\bSigma_{\tilde\xb, r, a}^{(t)}-\bigg[\frac{1}{t}\sum_{\tau\in[t]}\pi_{\tau}^{nd}(a)\xb_\tau \xb_{\tau}^\top\bigg]\btheta^*_{a}\bigg\|_2\geq 64R\max\left\{\frac{d+\log t}{q_tt}, \sqrt{\frac{d+\log t}{q_tt}}\right\}\right)\leq \frac{2}{t^2}.
\end{equation}
Combining (\ref{eq:hat-Sigma-x-r-2}) and (\ref{eq:hat-Sigma-x-2}), we conclude the proof.

\subsection{Proof of Corollary \ref{cor:alg1-with-theta-estimation-S}}\label{pf:cor:alg1-with-theta-estimation-S}

In Theorem \ref{thm-regret-S}, choose $T_0 = \sqrt{T}/\alpha$. Then $\forall t>T_0$, $s_t\geq \alpha t>\sqrt{T}$. Moreover, it's easy to verify that as long as $T\geq \max\{10, \frac{C'[d+\log(\sqrt{T})]^2}{\min\{\lambda_{0}^2, \lambda_{0}^4\}p_0^2}\}$ with $C'=C_1^2$ as in Theorem \ref{thm:theta-estimation}, $\forall t\geq \sqrt{T}$, $t\geq \frac{C_t}{\min\{\lambda_{0}, \lambda_{0}^2\}}\frac{d+\log t}{p_0}$. This implies that $\forall t>T_0$, $s_t\geq\max\{\sqrt{T}, \frac{C_1}{\min\{\lambda_{0}, \lambda_{0}^2\}}\frac{d+\log t}{p_0}\}$. Combining the results in Theorem \ref{thm-regret-S} and Theorem \ref{thm:theta-estimation}, we obtain that the regret of Algorithm \ref{alg2}
\begin{align*}
\text{Regret}(T)&\leq \frac{2}{\alpha}R_\theta\sqrt{T} + 2(1-2p_0)\sum_{t>\sqrt{T}/\alpha}\frac{C(R+R_\theta)}{\lambda_{0}} \max\left\{\frac{d+\log s_t}{p_0s_t}, \sqrt{\frac{d+\log s_t}{p_0s_t}}\right\}\\
&\leq \frac{2}{\alpha}R_\theta\sqrt{T} + \frac{2C(1-2p_0)(R+R_\theta)}{\lambda_{0}}\sum_{t>\sqrt{T}/\alpha} \max\left\{\frac{d+\log (\alpha t)}{p_0\alpha t}, \sqrt{\frac{d+\log (\alpha t)}{p_0\alpha t}}\right\}%\\
%&\leq \frac{2}{\alpha}R_\theta\sqrt{T} + \frac{2C(1-p_0)(R+R_\theta)}{\lambda_{\min}}\sum_{t>\sqrt{T}/\alpha} \max\left\{\frac{d+\log (\alpha t)}{p_0\alpha t}, \sqrt{\frac{d+\log (\alpha t)}{p_0\alpha t}}\right\}
\end{align*}
Here we use the fact that the mapping $u\mapsto \frac{d+\log u}{u}$ is monotonically decreasing on $[3,+\infty)$, and that $s_t\geq \alpha t> 3$ for all $t>\sqrt{T}/\alpha$ due to the assumptions in the corollary. Moreover, one can also verify that as long as $T\geq \max\{10, \frac{[d+\log(\sqrt{T})]^2}{p_0^2}\}$, we have $\forall t>\sqrt{T}/\alpha$, $\frac{d+\log (\alpha t))}{p_0\alpha t}\leq 1$. Thus, we can further deduce that
\begin{align}
\text{Regret}(T)
&\leq \frac{2}{\alpha}R_\theta\sqrt{T} + \frac{2C(1-2p_0)(R+R_\theta)}{\lambda_{0}}\sum_{t>\sqrt{T}/\alpha} \sqrt{\frac{d+\log (\alpha t)}{p_0\alpha t}}\nonumber\\
&\leq \frac{2}{\alpha}R_\theta\sqrt{T} + \frac{2C(1-2p_0)(R+R_\theta)}{\sqrt{p_0\alpha}\lambda_{0}}\left(\sqrt{d+\log \alpha }\cdot \sum_{t>\sqrt{T}/\alpha} \sqrt{\frac{1}{t}}+\sum_{t>\sqrt{T}/\alpha} \sqrt{\frac{\log t}{t}}\right).\label{eq:regret-analysis-w-estimation-S}
\end{align}

Plug (\ref{eq-integral-analysis1}) and (\ref{eq-integral-analysis2}) into (\ref{eq:regret-analysis-w-estimation-S}), we deduce that
\begin{align*}
\text{Regret}(T)
&\leq \frac{2}{\alpha}R_\theta\sqrt{T} + \frac{2C(1-2p_0)(R+R_\theta)}{\sqrt{p_0\alpha}\lambda_{0}}\left(\sqrt{d+\log \alpha }\cdot2\sqrt{T}+2\sqrt{T\log T}\right)\\
&\leq \frac{2}{\alpha}R_\theta\sqrt{T} + \frac{4C(1-2p_0)(R+R_\theta)}{\sqrt{p_0\alpha}\lambda_{0}}\sqrt{T}\left(\sqrt{d+\log \alpha}+\sqrt{\log T}\right),
\end{align*}
from which we conclude the proof.
